# Supplementary material for: First double-differential cross section measurement of neutral-current $\pi^0$ production in neutrino-argon scattering in the MicroBooNE detector
Source: arXiv:2404.10948 ancillary file (2025-03-31)
Supplement: Supplementary file 1 [file SupMat_PRL_NCpi0_v3.3.4.pdf]

# Supplemental Material for "First double-differential cross section measurement of neutral-current $\pi^0$ production in neutrino-argon scattering in the MicroBooNE detector"

## I. EFFICIENCIES AND PURITIES

This section shows the purities and efficiencies for the chosen binning schemes and 35 MeV kinetic energy threshold used to divide the 0p and Np channels. The overall efficiency and the purity for the sample of events fully-contained (FC) within the detector are shown for all measurements presented in Sec. IX. For the simultaneous 0p and Np measurements, the efficiency and purity with respect to (w.r.t.) the NC$\pi^0$ selection are also shown. These are defined by the ratio of the number of true 0p signal events selected as 0p to the total number of true 0p signal events passing the NC$\pi^0$ selection (total number of true signal events, with no requirement on protons, selected as 0p). The definitions of these metrics are written out explicitly Eq. (1) - (10). Examining these two sets of metrics is useful in separating the impact of the split into 0p and Np subchannels from the overall NC$\pi^0$ selection. Put another way, for 0p (Np) events, the efficiency w.r.t. NC$\pi^0$ is the probability that a true NC$\pi^0$ 0p (Np) event selected by the NC$\pi^0$ selection is categorised correctly as reconstructed 0p (Np), whereas the overall efficiency is the probability that any true 0p (Np) NC$\pi^0$ event is selected as a reconstructed 0p (Np) NC$\pi^0$ event. Similarly, the purity w.r.t. NC$\pi^0$ is the probability that a true NC$\pi^0$ event that passes the reconstructed NC$\pi^0$ 0p (Np) selection is really a true $\pi^0$ 0p (Np) event, whereas the overall purity is the probability any reconstructed 0p (Np) selected event is a true NC$\pi^0$ 0p (Np) event. In the following figures, the same binning is used for the purity as the efficiency, with the only exception being the highest $P_{\pi^0}$ bin, which corresponds to overflow in reconstructed space but ends at 1200 MeV in truth space.

$$\text{Xp efficiency} = \frac{\text{Number of true NC}\pi^0\text{ events selected as NC}\pi^0}{\text{Number of true NC}\pi^0\text{ events}} \tag{1}$$

$$\text{Np efficiency} = \frac{\text{Number of true NC}\pi^0\text{ Np events selected as NC}\pi^0\text{ Np}}{\text{Number of true Np NC}\pi^0\text{ events}} \tag{2}$$

$$\text{0p efficiency} = \frac{\text{Number of true NC}\pi^0\text{ 0p events selected as NC}\pi^0\text{ 0p}}{\text{Number of true 0p NC}\pi^0\text{ events}} \tag{3}$$

$$\text{Np efficiency w.r.t. NC}\pi^0\text{ selection} = \frac{\text{Number of true NC}\pi^0\text{ Np events selected as NC}\pi^0\text{ Np}}{\text{Number of true NC}\pi^0\text{ Np events selected as NC}\pi^0} \tag{4}$$

$$\text{0p efficiency w.r.t. NC}\pi^0\text{ selection} = \frac{\text{Number of true NC}\pi^0\text{ 0p events selected as NC}\pi^0\text{ 0p}}{\text{Number of true NC}\pi^0\text{ 0p events selected as NC}\pi^0} \tag{5}$$

$$\text{Xp purity} = \frac{\text{Number of true NC}\pi^0\text{ events selected as NC}\pi^0}{\text{Number of events selected as NC}\pi^0} \tag{6}$$

$$\text{Np purity} = \frac{\text{Number of true NC}\pi^0\text{ Np events selected as NC}\pi^0\text{ Np}}{\text{Number of events selected as NC}\pi^0\text{ Np}} \tag{7}$$

$$\text{0p purity} = \frac{\text{Number of true NC}\pi^0\text{ 0p events selected as NC}\pi^0\text{ 0p}}{\text{Number of events selected as NC}\pi^0\text{ 0p}} \tag{8}$$

$$\text{Np purity w.r.t. NC}\pi^0\text{ selection} = \frac{\text{Number of true NC}\pi^0\text{ Np events selected as NC}\pi^0\text{ Np}}{\text{Number of true NC}\pi^0\text{ events selected as NC}\pi^0\text{ Np}} \tag{9}$$

$$\text{0p purity w.r.t. NC}\pi^0\text{ selection} = \frac{\text{Number of true NC}\pi^0\text{ 0p events selected as NC}\pi^0\text{ 0p}}{\text{Number of true NC}\pi^0\text{ events selected as NC}\pi^0\text{ 0p}} \tag{10}$$

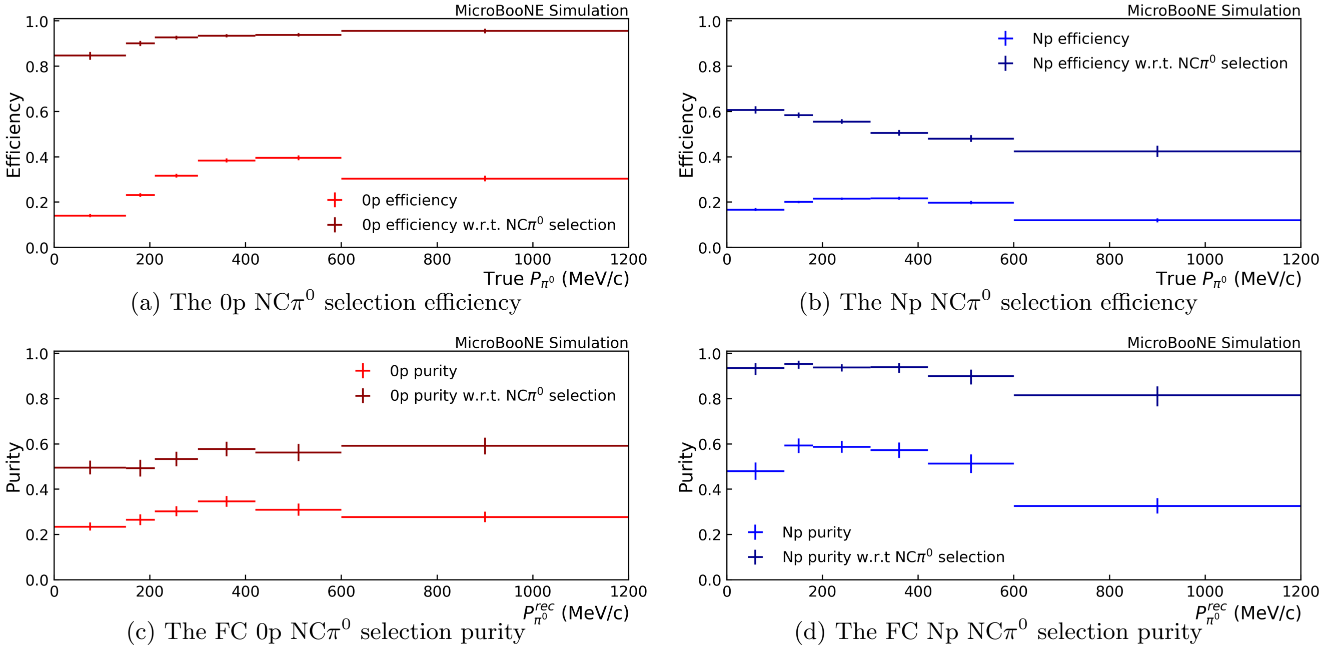


(a) The 0p NC$\pi^0$ selection efficiency

(b) The Np NC$\pi^0$ selection efficiency

(c) The FC 0p NC$\pi^0$ selection purity

(d) The FC Np NC$\pi^0$ selection purity

FIG. 1: [(a) and (b)] The 0p and Np NC$\pi^0$ selection efficiency as a function of true $\pi^0$ momentum. [(c) and (d)] The 0p and Np NC$\pi^0$ selection purity as a function of reconstructed $\pi^0$ momentum for FC events. The error bars contain only statistical uncertainty. The 0p (Np) efficiency w.r.t. NC$\pi^0$ and purity w.r.t NC$\pi^0$ are calculated using only true 0p (Np) signal events passing the NC$\pi^0$ selection. The last bin ends at 1200 MeV in (a) and (b), but is treated as overflow in (c) and (d).

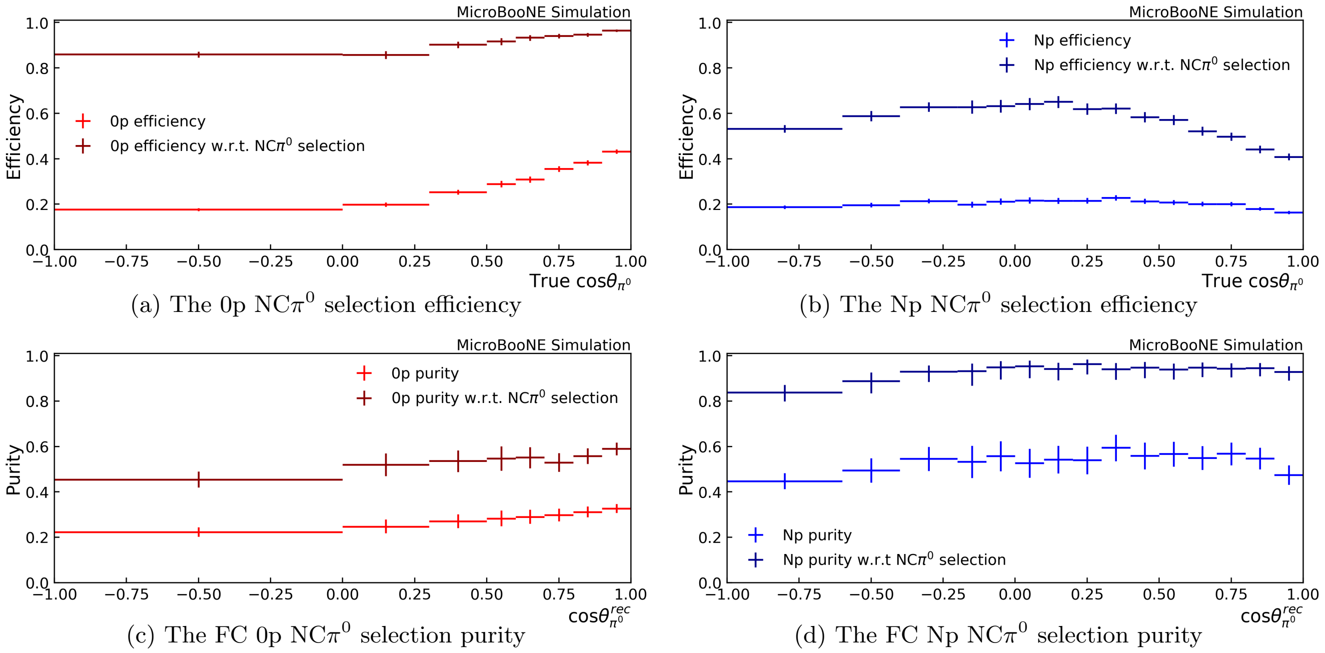


(a) The 0p NC$\pi^0$ selection efficiency

(b) The Np NC$\pi^0$ selection efficiency

(c) The FC 0p NC$\pi^0$ selection purity

(d) The FC Np NC$\pi^0$ selection purity

FIG. 2: [(a) and (b)] The 0p and Np NC$\pi^0$ selection efficiency as a function of true $\cos\theta_{\pi^0}$. [(c) and (d)] The 0p and Np NC$\pi^0$ selection purity as a function of reconstructed $\cos\theta_{\pi^0}$ for FC events. The error bars contain only statistical uncertainty. The 0p (Np) efficiency w.r.t. NC$\pi^0$ and purity w.r.t. NC$\pi^0$ are calculated using only true 0p (Np) signal events passing the NC$\pi^0$ selection.

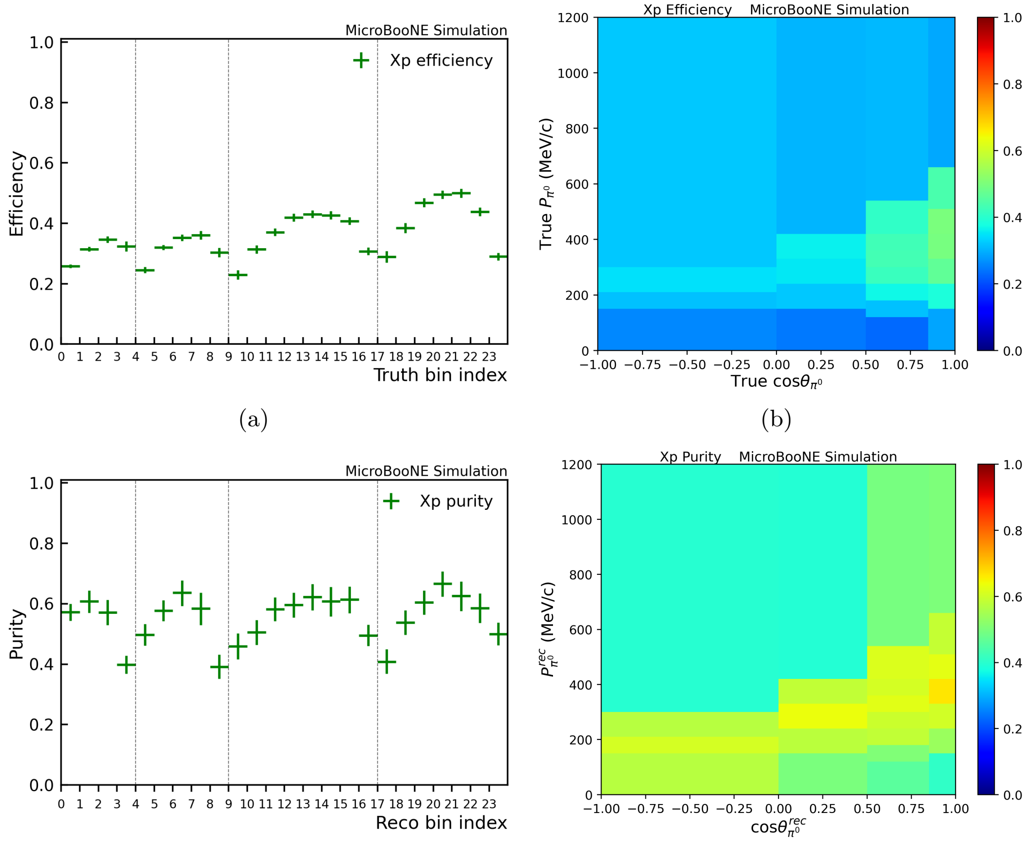


(a) (b) (c) (d)

FIG. 3: [(a) and (b)] The Xp NC$\pi^0$ selection efficiency as a function of true $\cos\theta_{\pi^0}$ and $P_{\pi^0}$. [(c) and (d)] The Xp NC$\pi^0$ selection purity as a function of reconstructed $\cos\theta_{\pi^0}$ and $P_{\pi^0}$ for FC events. In (b) and (d) the bins are displayed according to the physical bin width with the z axis indicating the efficiency (purity). In (a) and (c) the bins are vectorized as a function of the bin width with error bars containing only statistical uncertainty. The y axis thus corresponds to the efficiency (purity) and the bins do not correspond to their physical width. The same binning is used for the purity and the efficiency, with the only exception being the last bin of each angular slice, which correspond to overflow in reconstructed space but end at 1200 MeV in truth space. More information on the binning can be found in Sec. IX.

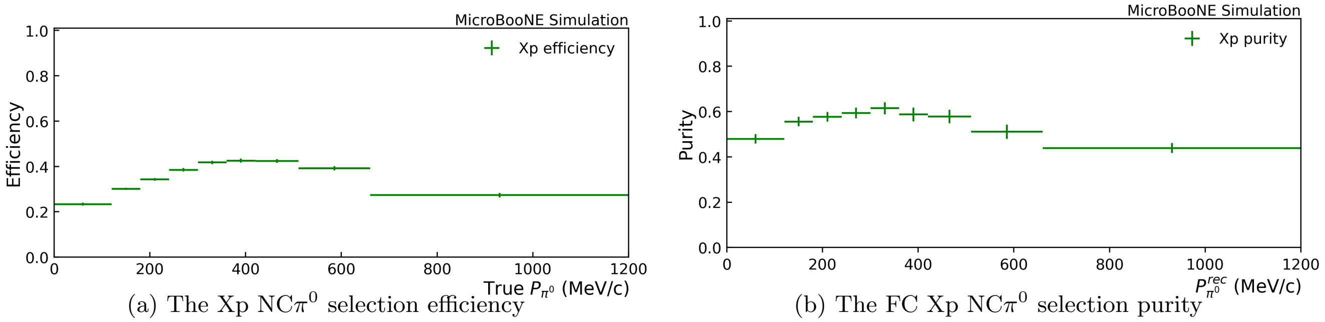


(a) The Xp NC$\pi^0$ selection efficiency

(b) The FC Xp NC$\pi^0$ selection purity

FIG. 4: (a) The Xp NC$\pi^0$ selection efficiency as a function of true $\pi^0$ momentum. (b) The Xp NC$\pi^0$ selection purity as a function of reconstructed $\pi^0$ momentum for FC events. The error bars contain only statistical uncertainty. The last bin ends at 1200 MeV in (a), but is treated as overflow in (b).

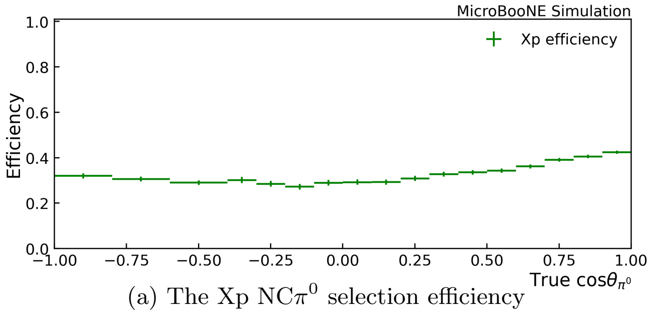


(a) The Xp NC$\pi^0$ selection efficiency

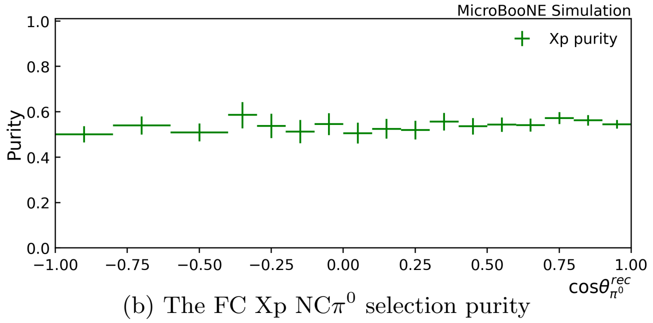


(b) The FC Xp NC$\pi^0$ selection purity

FIG. 5: (a) The Xp NC$\pi^0$ selection efficiency as a function of true $\cos\theta_{\pi^0}$. (b) The Xp NC$\pi^0$ selection purity as a function of reconstructed $\cos\theta_{\pi^0}$ for FC events. The error bars contain only statistical uncertainty.

## II. SMEARING MATRICES

The following figures show the smearing between reconstructed and true bins. This illustrates the reconstruction quality and degree to which the overall model must correct for imperfect reconstruction. These histograms contain all FC selected signal events with each column normalized to one. Thus, a given bin describes the probability that a selected signal event in the corresponding truth bin will be reconstructed in the corresponding reconstructed space bin. The sliced measurements and simultaneous 0p and Np measurements contain separate blocks for each slice/multiplicity. Events are categorized as reconstructed (true) Np if they have a reconstructed (true) primary proton with kinetic energy greater than 35 MeV. In these figures, the same binning was used for reconstructed space and truth space, with the only exception being the last $P_{\pi^0}$ bin, which corresponds to overflow in reconstructed space but ends at 1.2 GeV/c in truth space. The most prominent smearing comes from true Np events which are reconstructed as 0p. Beyond this, the histograms in this section are mostly diagonal, indicating relatively good reconstruction quality on the variables of interest.

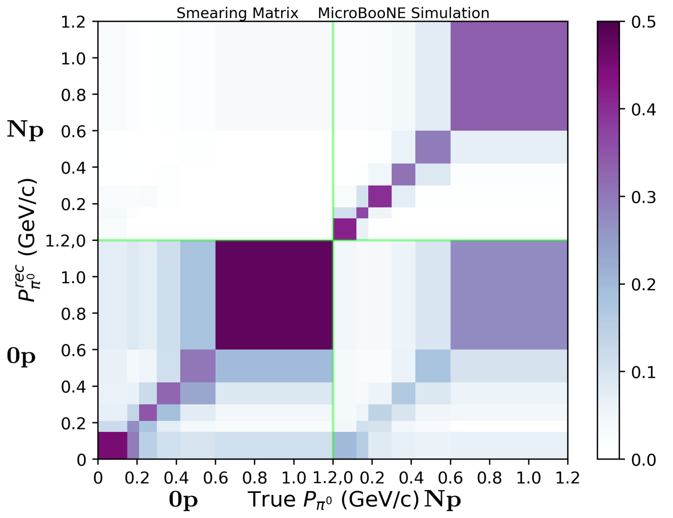


(a) 0p and Np $P_{\pi^0}$ smearing matrix

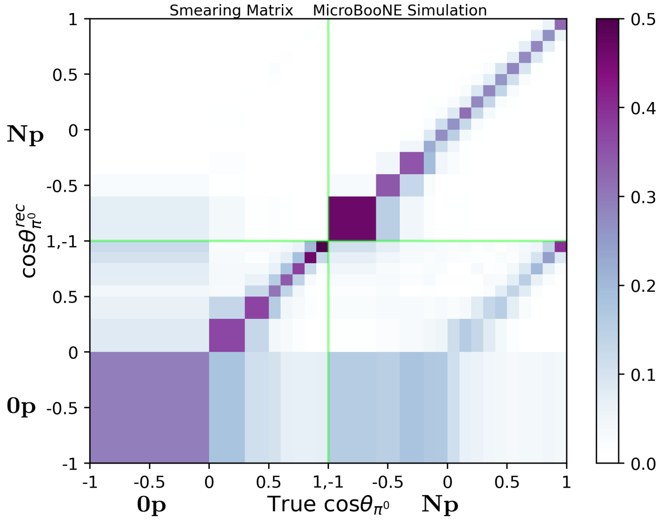


(b) 0p and Np $\cos\theta_{\pi^0}$ smearing matrix

FIG. 6: Smearing matrices for the simultaneous 0p and Np (a) single-differential $P_{\pi^0}$ and (b) single-differential $\cos\theta_{\pi^0}$ measurements. Selected FC signal events are shown with each column normalized to one. The green lines divide bins containing true (reconstructed) events with and without protons, where reconstructed 0p (Np) and true 0p (Np) is on the bottom (top) left (right), and reconstructed 0p (Np) and true Np (0p) is on the bottom (top) right (left). In (a), the last bin of each multiplicity block corresponds to overflow in reconstructed space but ends at 1.2 GeV/c in truth space.

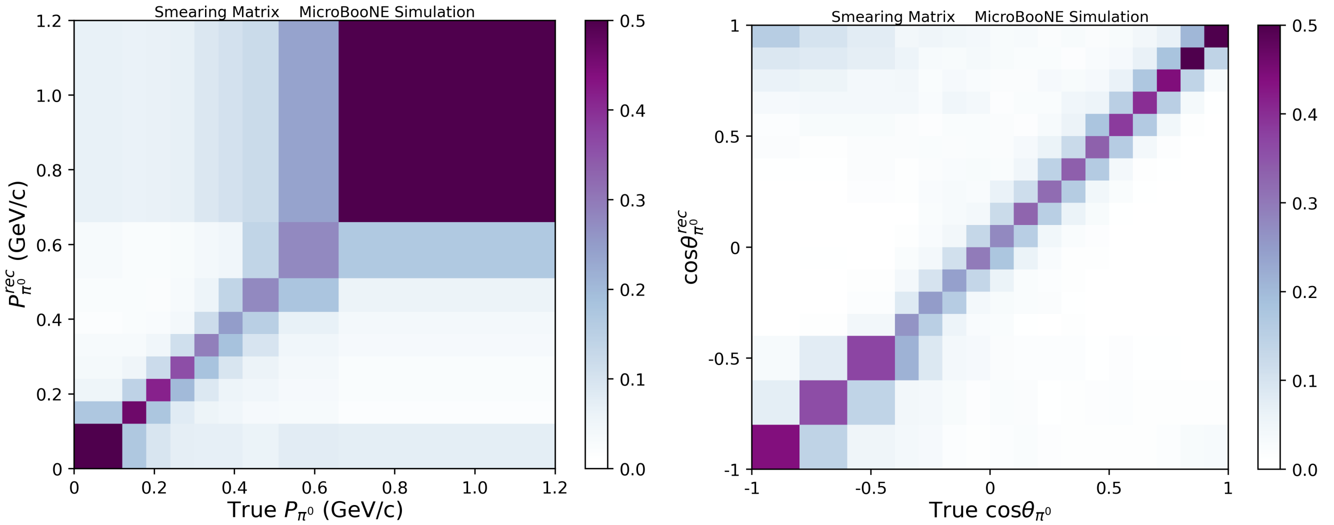


(a) Xp $P_{\pi^0}$ smearing matrix

(b) Xp $\cos\theta_{\pi^0}$ smearing matrix

FIG. 7: Smearing matrices for the Xp (a) single-differential $P_{\pi^0}$ and (b) single-differential $\cos\theta_{\pi^0}$ measurements. Selected FC signal events are shown with each column normalized to one. In (a), the last bin corresponds to overflow in reconstructed space but ends at 1.2 GeV/c in truth space.

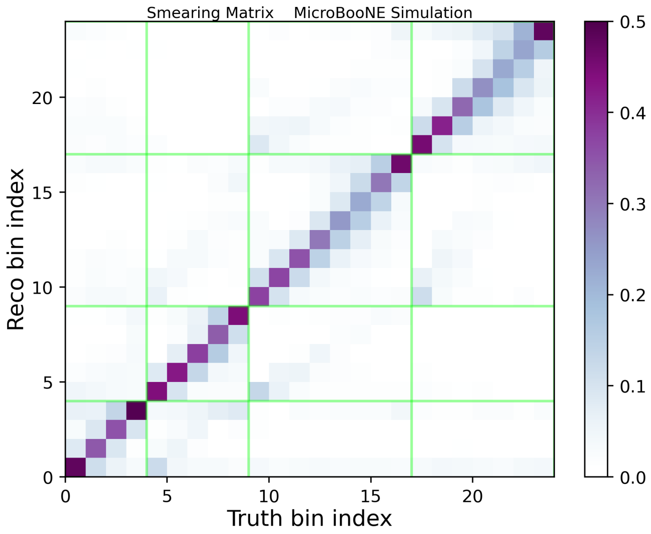


FIG. 8: Smearing matrix for the Xp double-differential $\cos\theta_{\pi^0}$ and $P_{\pi^0}$ measurement. Selected FC signal events are shown with each column normalized to one. The axes corresponds to the bin index. As such, the bins do not correspond to their physical width. The green lines indicate the division between angular slices. The binning is the same for reconstructed space as truth space, with the only exception being the last bin of all angular slices, which correspond to overflow in reconstructed space but end at 1.2 GeV/c in truth space. More information on the binning can be found in Sec. IX.

## III. UNCERTAINTIES ON EXTRACTED RESULTS

What follows is the contribution of uncertainties by systematic type and the corresponding covariance and correlation matrices for each extracted cross section. Note that these correlation and covariance matrices have axes corresponding to the bin index and all bins are equal width rather than their physical width. For the 0p and Np figures, the 0p bins all come before the Np ones. For the double-differential measurement, the bins are in angular slices, which go from backwards on the left to forwards on the right. The binning is described in more detail in Sec. IX. In all cases, the detector systematics are the dominant source of uncertainty. This is followed by the data statistical, flux and cross section uncertainties which all contribute at comparable levels. The data statistical uncertainties tend to be the largest of these three except in regions with a larger numbers of events, such as moderate momenta and forward angles. MC statistical, dirt, POT, target and reinteraction systematics are all sub-dominant and contribute little to the total uncertainty. The total uncertainty is larger at higher momenta in all measurements. It is also somewhat larger at backwards angles for 0p and Xp, while appearing relatively flat across all angles for Np.

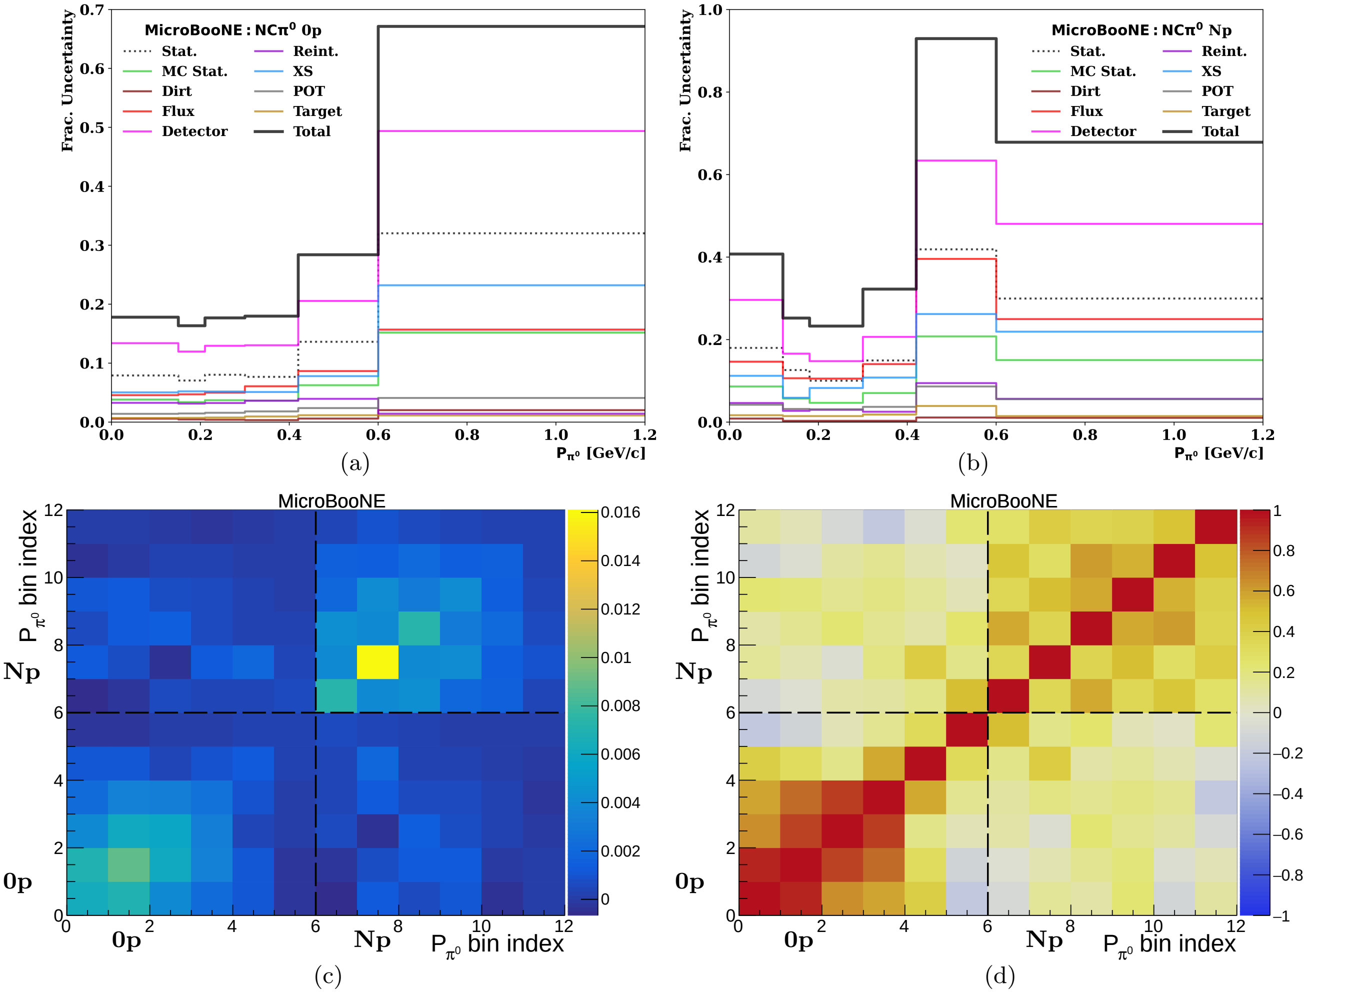


FIG. 9: Contribution of uncertainties by systematic type for the extraction of the (a) 0p and (b) Np $P_{\pi^0}$ differential cross section. (c) The covariance and (d) correlation matrices obtained from the simultaneous extraction of the 0p and Np $P_{\pi^0}$ differential cross section. The dashed lines separate the 0p and Np channels. On all subfigures, the true bins are those found in Sec. IX and are the same as those for the extracted cross section. The entries shown in (a) and (b) correspond to the square root of the diagonal elements of (c) divided by the value of the extracted cross section for the given bin. The covariance matrix in (c) is in units of $\left(10^{-39}\ \mathrm{cm}^2/\mathrm{nucleon}/(\mathrm{GeV/c})\right)^2$.

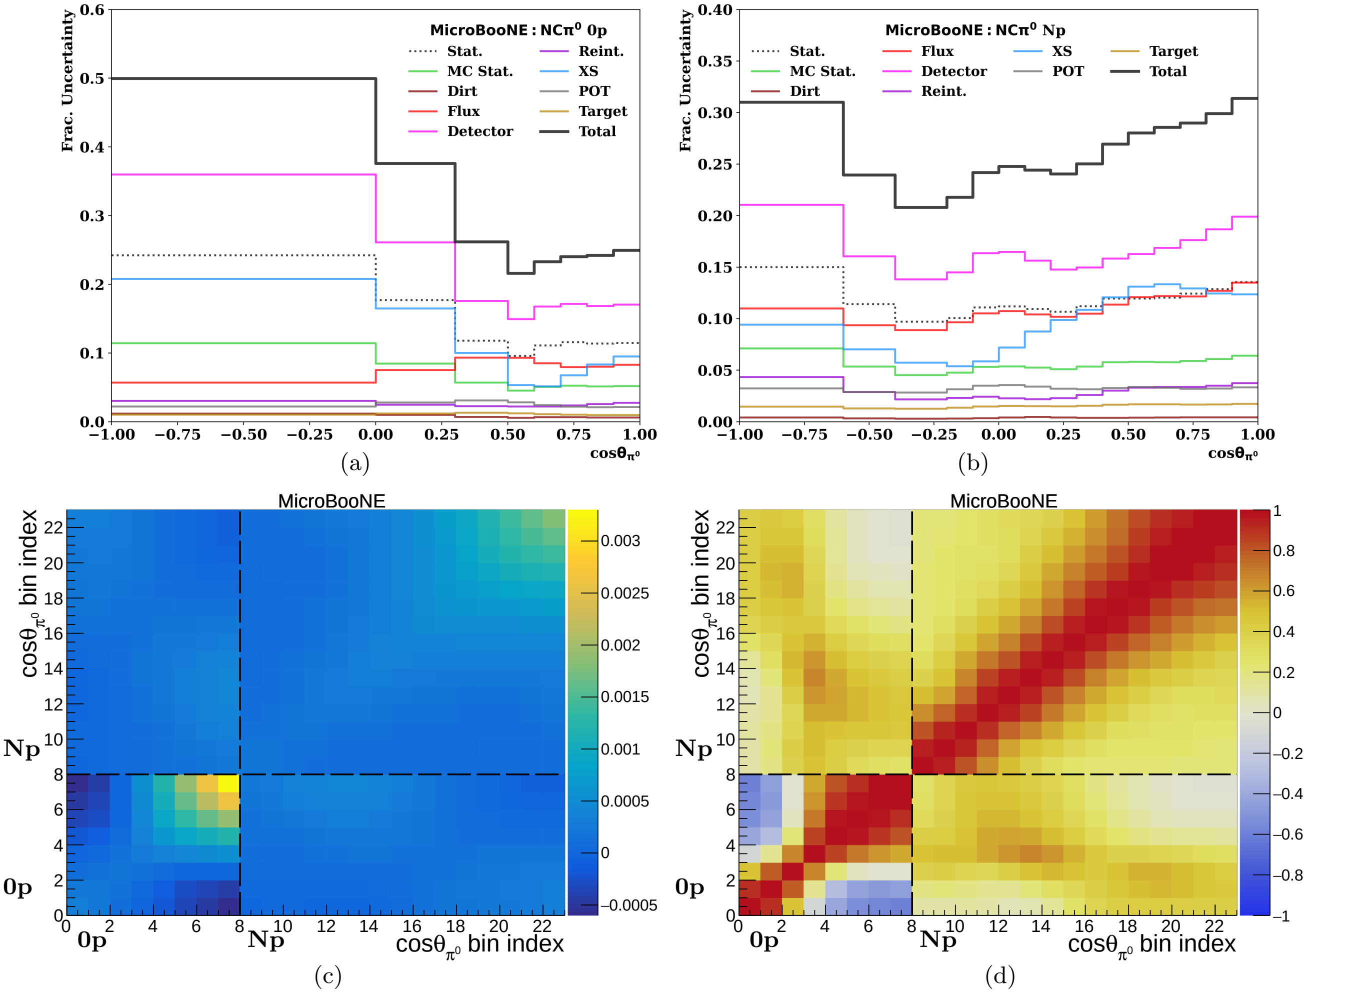


FIG. 10: Contribution of uncertainties by systematic type for the extraction of the (a) 0p and (b) Np $\cos\theta_{\pi^0}$ differential cross section. (c) The covariance and (d) correlation matrices obtained from the simultaneous extraction of the 0p and Np $\cos\theta_{\pi^0}$ differential cross section. The dashed lines separate the 0p and Np channels. On all subfigures, the true bins are those found in Sec. IX and are the same as those for the extracted cross section. The entries shown in (a) and (b) correspond to the square root of the diagonal elements of (c) divided by the value of the extracted cross section for the given bin. The covariance matrix in (c) is in units of $\left(10^{-39}\ \mathrm{cm}^2/\mathrm{nucleon}\right)^2$.

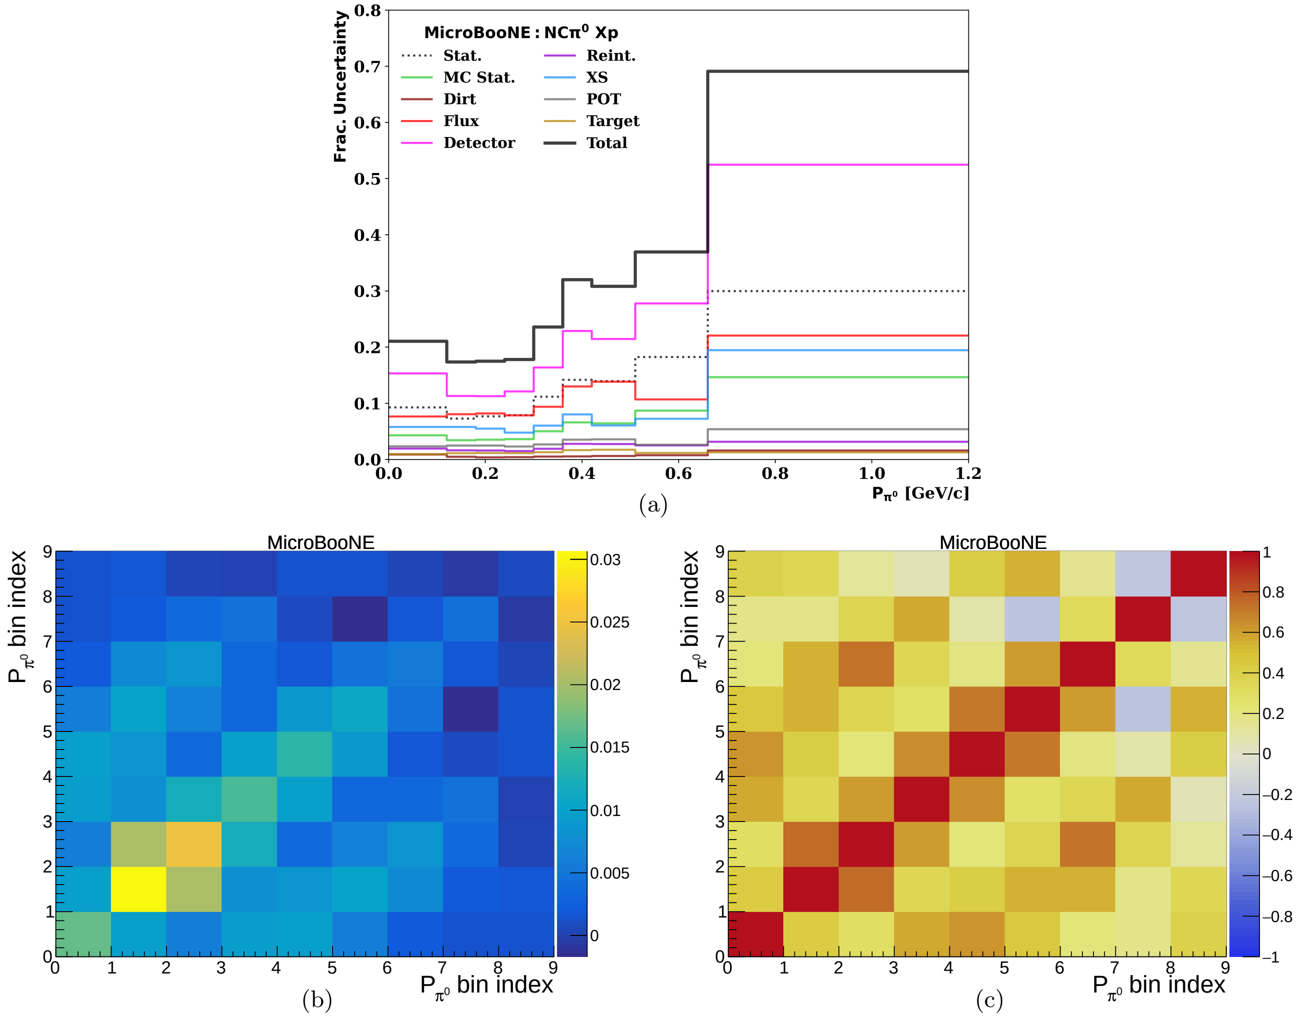


FIG. 11: (a) Contribution of uncertainties by systematic type for the extraction of the Xp $P_{\pi^0}$ differential cross section. (b) The covariance and (c) correlation matrices obtained from the extraction of the Xp $P_{\pi^0}$ differential cross section. On all subfigures, the true bins are those found in Sec. IX and are the same as those for the extracted cross section. The entries shown in (a) correspond to the square root of the diagonal elements of (b) divided by the extracted cross section for the given bin. The covariance matrix in (b) is in units of $\left(10^{-39}\ \mathrm{cm}^2/\mathrm{nucleon}/(\mathrm{GeV/c})\right)^2$.

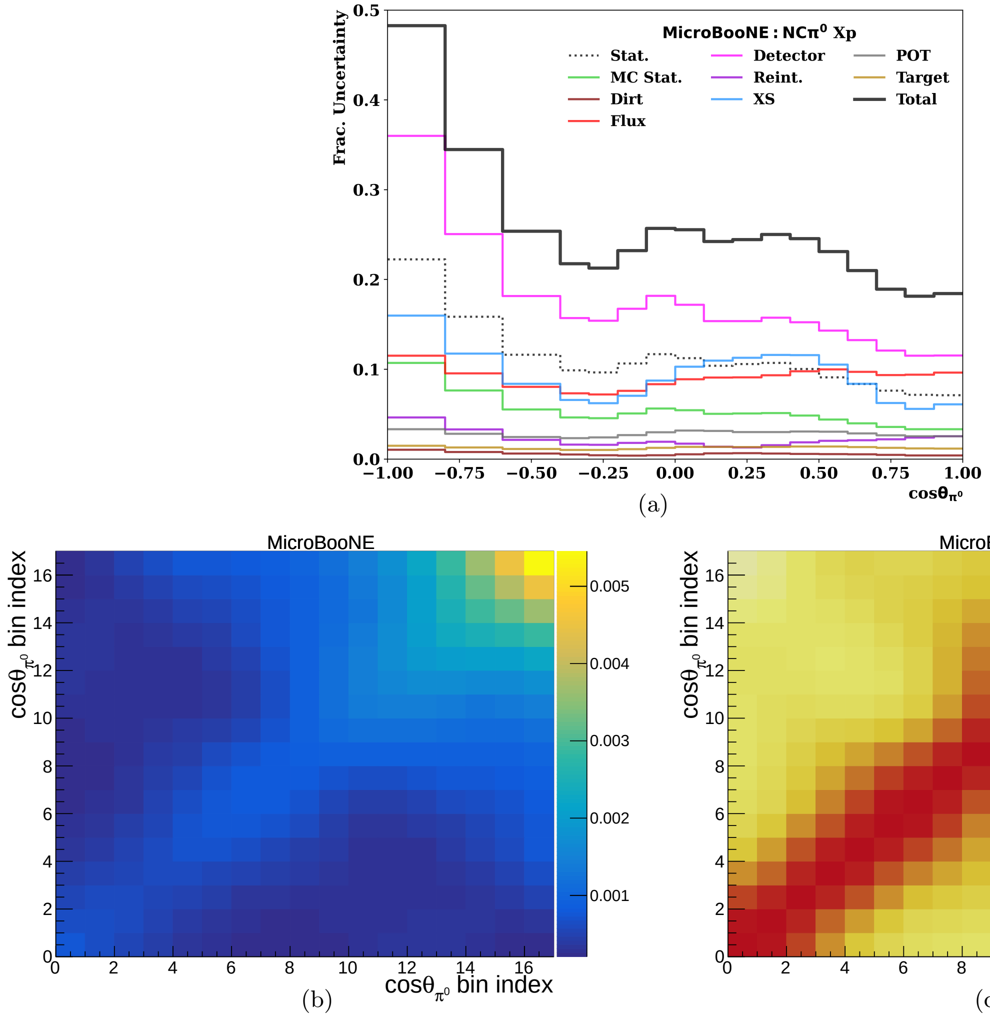


FIG. 12: (a) Contribution of uncertainties by systematic type for the extraction of the Xp $\cos\theta_{\pi^0}$ differential cross section. (b) The covariance and (c) correlation matrices obtained from the extraction of the Xp $\cos\theta_{\pi^0}$ differential cross section. On all subfigures, the true bins are those found in Sec. IX and are the same as those on the extracted cross section. The entries shown in (a) correspond to the square root of the diagonal elements of (b) divided by the extracted cross section for the given bin. The covariance matrix in (c) is in units of $\left(10^{-39}\ \text{cm}^2/\text{nucleon}\right)^2$.

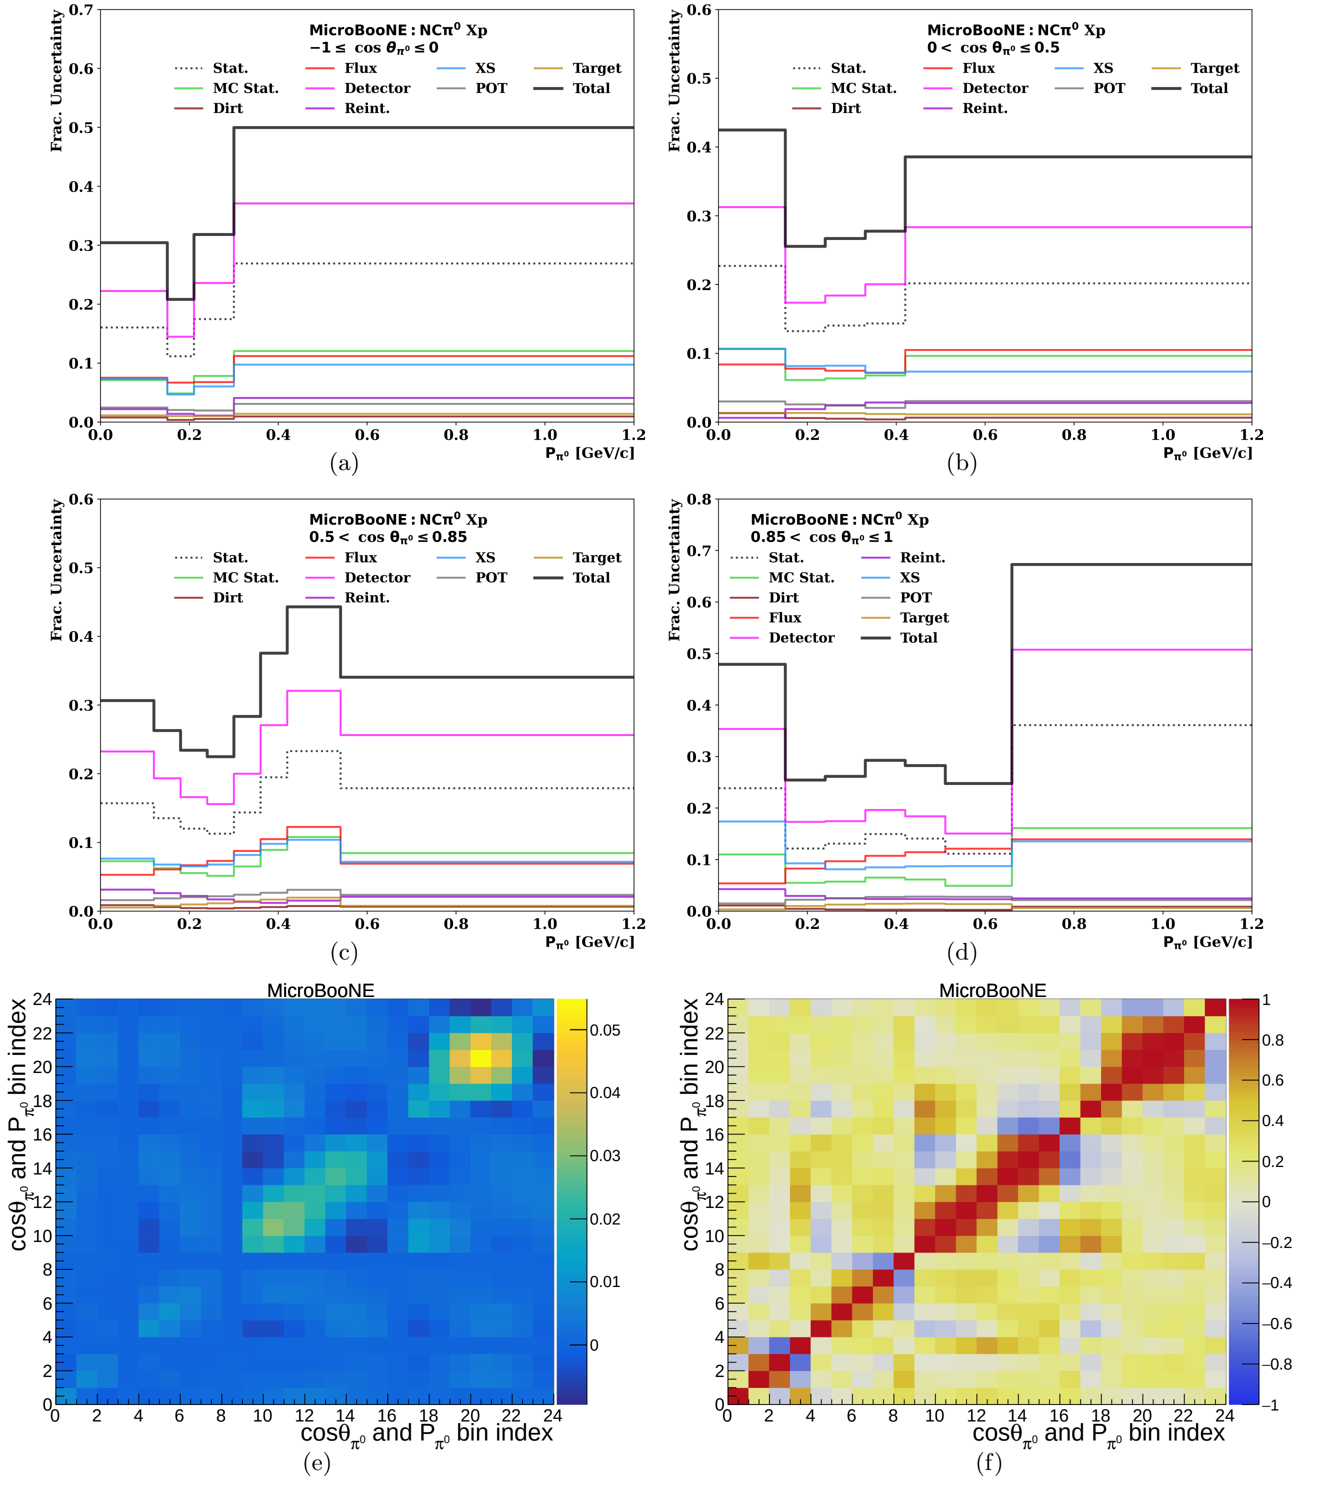


FIG. 13: (a)-(d) Contribution of uncertainties by systematic type for the extraction of the Xp $\cos\theta_{\pi^0}$ and $P_{\pi^0}$ double-differential cross section. Different angular regions are shown in each subfigure. (e) The covariance and (f) correlation matrices obtained from the extraction of the Xp $\cos\theta_{\pi^0}$ and $P_{\pi^0}$ double-differential cross section. On all subfigures, the true bins are those found in Sec. IX and are the same as those for the extracted cross section. In (e) and (f), the bins are in angular slices, which go from backwards on the left to forwards on the right. The entries shown in (a)-(d) correspond to the square root of the diagonal elements of (e) divided by the value of the extracted cross section for the given bin. The covariance matrix in (e) is in units of $(10^{-39}\ \mathrm{cm}^2/\mathrm{nucleon}/(\mathrm{GeV/c}))^2$.

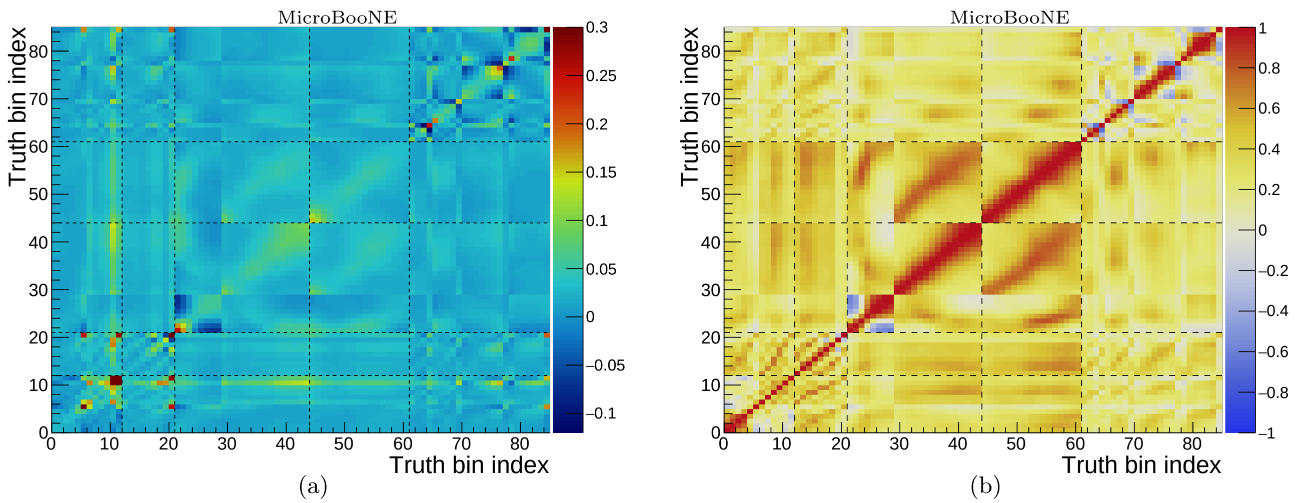


FIG. 14: The blockwise (a) fractional covariance and (b) correlation matrices obtained utilizing the blockwise unfolding procedure. The dashed lines separate different measurements which are ordered as follows: 0p and Np $P_{\pi^0}$, Xp $P_{\pi^0}$, 0p and Np $\cos\theta_{\pi^0}$, Xp $\cos\theta_{\pi^0}$, and Xp $\{\cos\theta_{\pi^0}, P_{\pi^0}\}$. Each axis corresponds to the bin index and does not represent the physical width of the bin. More information on the binning is found in Sec. IX.

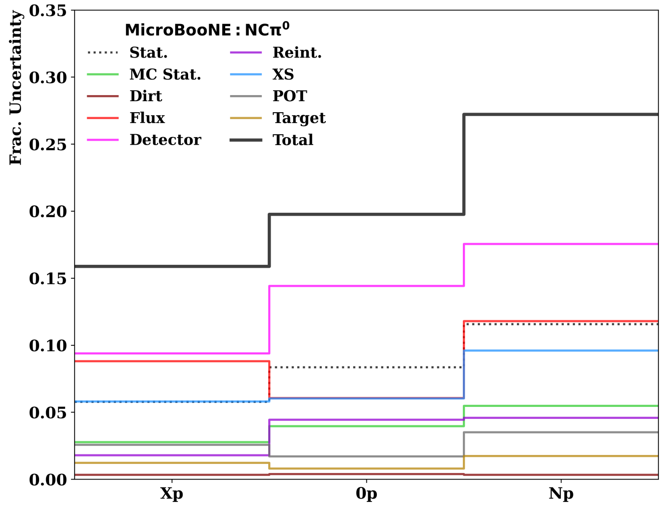


FIG. 15: Contribution of uncertainties by systematic type for the total Xp, 0p, and Np cross sections.

## IV. ADDITIONAL SMEARING MATRICES $A_C$

This section contains the additional smearing matrices, $A_C$, obtained in the Wiener-SVD unfolding. These matrices capture the bias induced by regularization. Any generator or theory prediction should be multiplied by this matrix when making a comparison to this data. For the simultaneous 0p and Np measurements, the 0p bins all come before the Np ones. For the double-differential measurement, the bins are in angular slices, which go from backwards on the left to forwards on the right. The binning is described in more detail in Sec. IX.

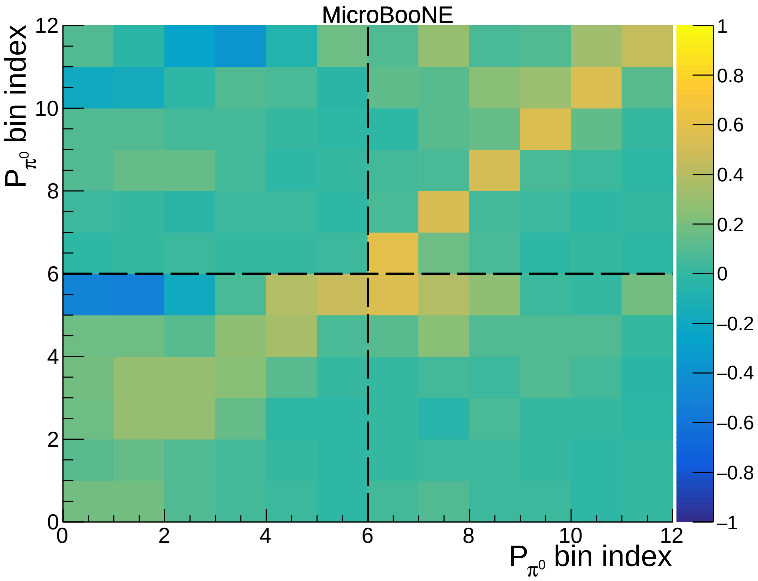


FIG. 16: The additional smearing matrix, $A_C$, obtained from the simultaneous extraction of the the 0p and Np $P_{\pi^0}$ differential cross section. The dashed lines separate the 0p and Np channels. The true bins are those found in Sec. IX and are the same as those for the extracted cross section.

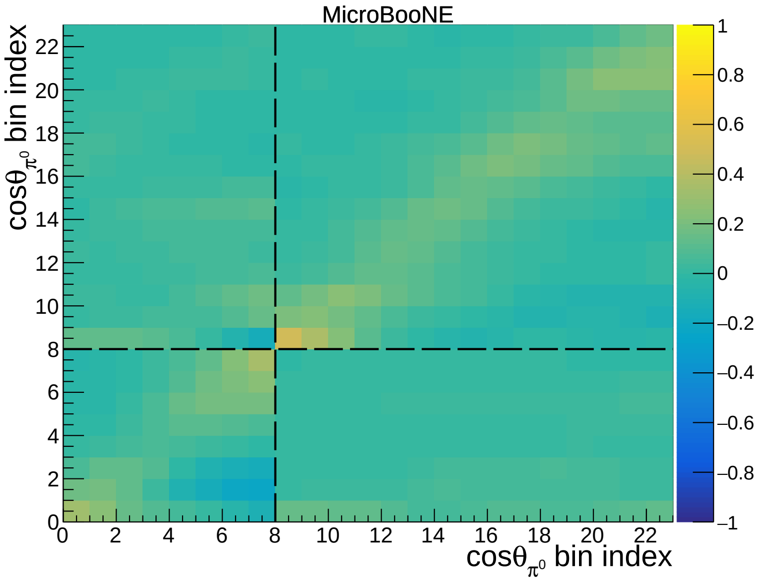


FIG. 17: The additional smearing matrix, $A_C$, obtained from the simultaneous extraction of the the 0p and Np $\cos\theta_{\pi^0}$ differential cross section. The dashed lines separate the 0p and Np channels. The true bins are those found in Sec. IX and are the same as those for the extracted cross section.

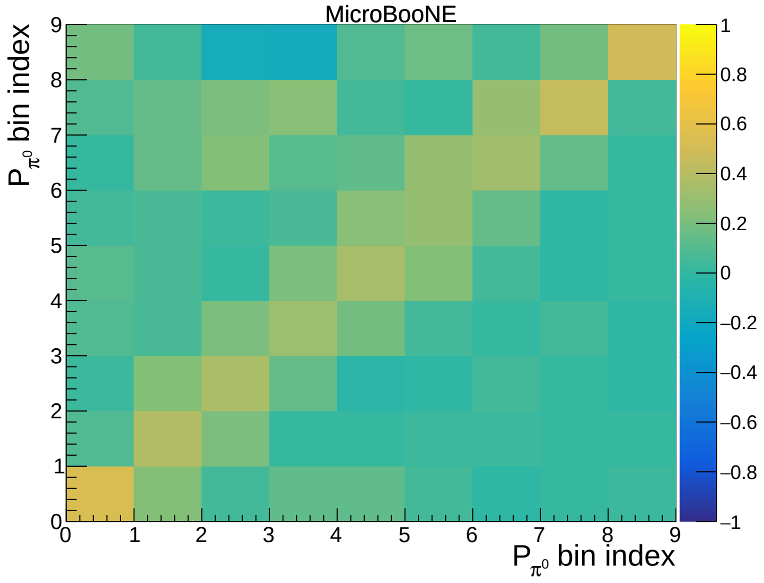


FIG. 18: The additional smearing matrix, $A_C$, obtained from the extraction of the the Xp $P_{\pi^0}$ differential cross section. The true bins are those found in Sec. IX and are the same as those for the extracted cross section.

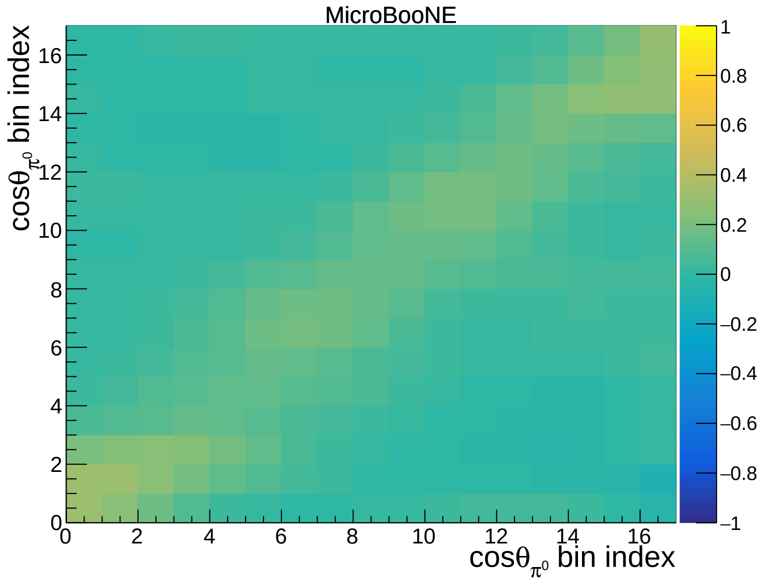


FIG. 19: The additional smearing matrix, $A_C$, obtained from the extraction of the the Xp $\cos\theta_{\pi^0}$ differential cross section. The true bins are those found in Sec. IX and are the same as those for the extracted cross section.

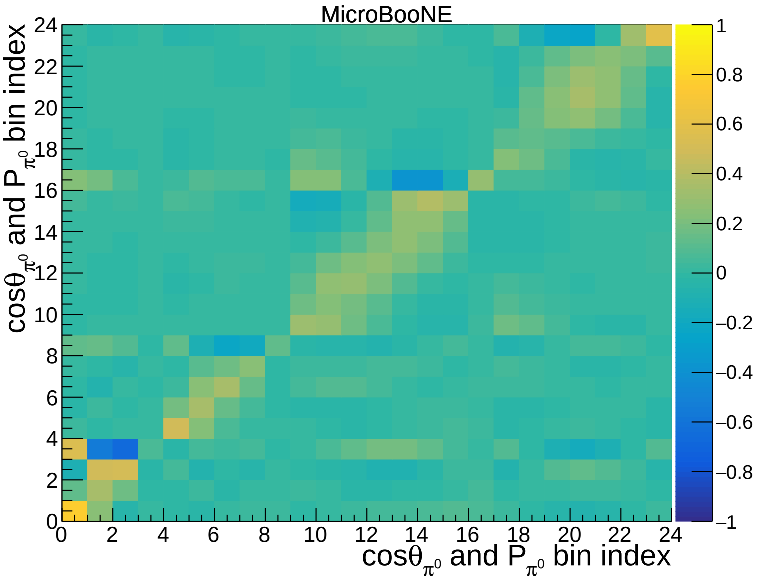


FIG. 20: The additional smearing matrix, $A_C$, obtained from the extraction of the the Xp $\cos\theta_{\pi^0}$ and $P_{\pi^0}$ differential cross section. The bining structure utilizes angle slices, which go from backwards on the left to forwards on the right. The true bins are those found in Sec. IX and are the same as those for the extracted cross section.

## V. MODEL VALIDATION

The following section contains the various tests used to validate the overall model used for cross section extraction, which is more briefly described in the main text. In these tests, the compatibility between the data and model is evaluated with goodness-of-fit tests that utilize a $\chi^2$ test statistic. Many of the tests also make use of the conditional constraint formalism [1] to increase the stringency of the validation. This procedure utilizes a set of data distributions to narrow the allowed model parameter space of a different set of distributions. The constraint does this by utilizing the correlations between these distributions, which describe the predicted relationship between them, alongside the observation in the constraining distribution to reduce the uncertainties and update the central value prediction on the constrained distribution. More explicitly, given a covariance matrix containing two channels (X, Y):

$$\Sigma = \begin{pmatrix} \Sigma^{XX} & \Sigma^{XY} \\ \Sigma^{YX} & \Sigma^{YY} \end{pmatrix}, \quad n : \text{measurement}, \quad \mu : \text{ prediction},$$

we can derive the prediction for $X$ given the constraints from $Y$,

$$\mu^{X,\text{const.}} = \mu^X + \Sigma^{XY} \cdot \left(\Sigma^{YY}\right)^{-1} \cdot \left(n^Y - \mu^Y\right)$$
$$\Sigma^{XX,\text{const.}} = \Sigma^{XX} - \Sigma^{XY} \cdot \left(\Sigma^{YY}\right)^{-1} \cdot \Sigma^{YX}.$$

Thus, by performing a goodness-of-fit test using the updated model prediction, $\mu^{X,\text{const.}}$, and the constrained model uncertainties of $\Sigma^{XX,\text{const.}}$, we achieve a more stringent examination of the compatibility between the model and data. This overall procedure follows closely what has been done in several other MicroBooNE analyses [2–4].

Specifically, for this analysis, the $\nu_\mu$CC selection (which is identical to that of [2–6]) is used to constrain the NC$\pi^0$ channel in the variables directly used in the unfolding and those relevant to the reconstruction of NC$\pi^0$ events. Several tests also utilize constraints directly from the NC$\pi^0$ selection but in other variables. Since, in these tests, the constraining and constrained distributions are formed from the same set of events, the correlations in the statistical uncertainties need to be accounted for. These correlations are estimated using a bootstrapping procedure to resample events and form a correlated statistical covariance matrix, which is added to the overall covariance matrix. To help ensure an unbiased unfolding, we require that the overall model is able to describe the data within $2\sigma$ for all tests.

The validation aims to test the model in the phase space relevant to the cross section extraction. It thus explores both 0p and Np final states and two dimensional $\{\cos\theta_{\pi^0}, P_{\pi^0}\}$ distributions. Quantities related to the reconstruction quality are also examined. The histograms shown in this section present the distributions of FC events. All model validation tests shown in this section are also applied to the PC distributions, which are less informative due to

their smaller event counts and larger uncertainties, and all of which yield a $p$-value close to one. This suite of tests demonstrates that the overall model is able to describe the data at the $2\sigma$ level. This indicates that any relevant mismodleing is covered by the stated uncertainties and the extracted cross sections will not be biased beyond the uncertainties obtained from the extracted covariance matrix.

Several histograms are shown with the MC prediction broken down into three signal categories and eight background categories. The background event categories are: "Cosmic", which corresponds to mistakenly selected cosmic-ray backgrounds selected in events for which a neutrino event is present; "EXT", which refers to cosmic-ray background events from the beam-off data set that have no BNB neutrino interactions; "Dirt", which refers to neutrino interactions with their true neutrino interaction vertices outside the cryostat; "Out FV", which includes events originating inside the cryostat but outside the fiducial volume (all subsequent categories require the event to be within the FV); "NC Other", which includes all NC interactions not part of the signal; "CC $\pi^0$" which corresponds to all $\nu_\mu$ (and $\bar{\nu}_\mu$) charged current events with a $\pi^0$, "CC Other" which comprises all $\nu_\mu$ (and $\bar{\nu}_\mu$) charged current events without a $\pi^0$; and "$\nu_e/\bar{\nu}_e$ CC", which includes all $\nu_e$ and $\bar{\nu}_e$ charged current events. The signal categories include all events in which a NC interaction of any flavor neutrino produces a single true $\pi^0$ with $P_{\pi^0} < 1.2$ GeV/c. Additionally, the "NC$\pi^0$ COH" category only includes signal events produced by a coherent process, "NC$\pi^0$ RES" includes only those from resonant pion production, and "NC$\pi^0$ Other" includes signal events not falling in the first two categories.

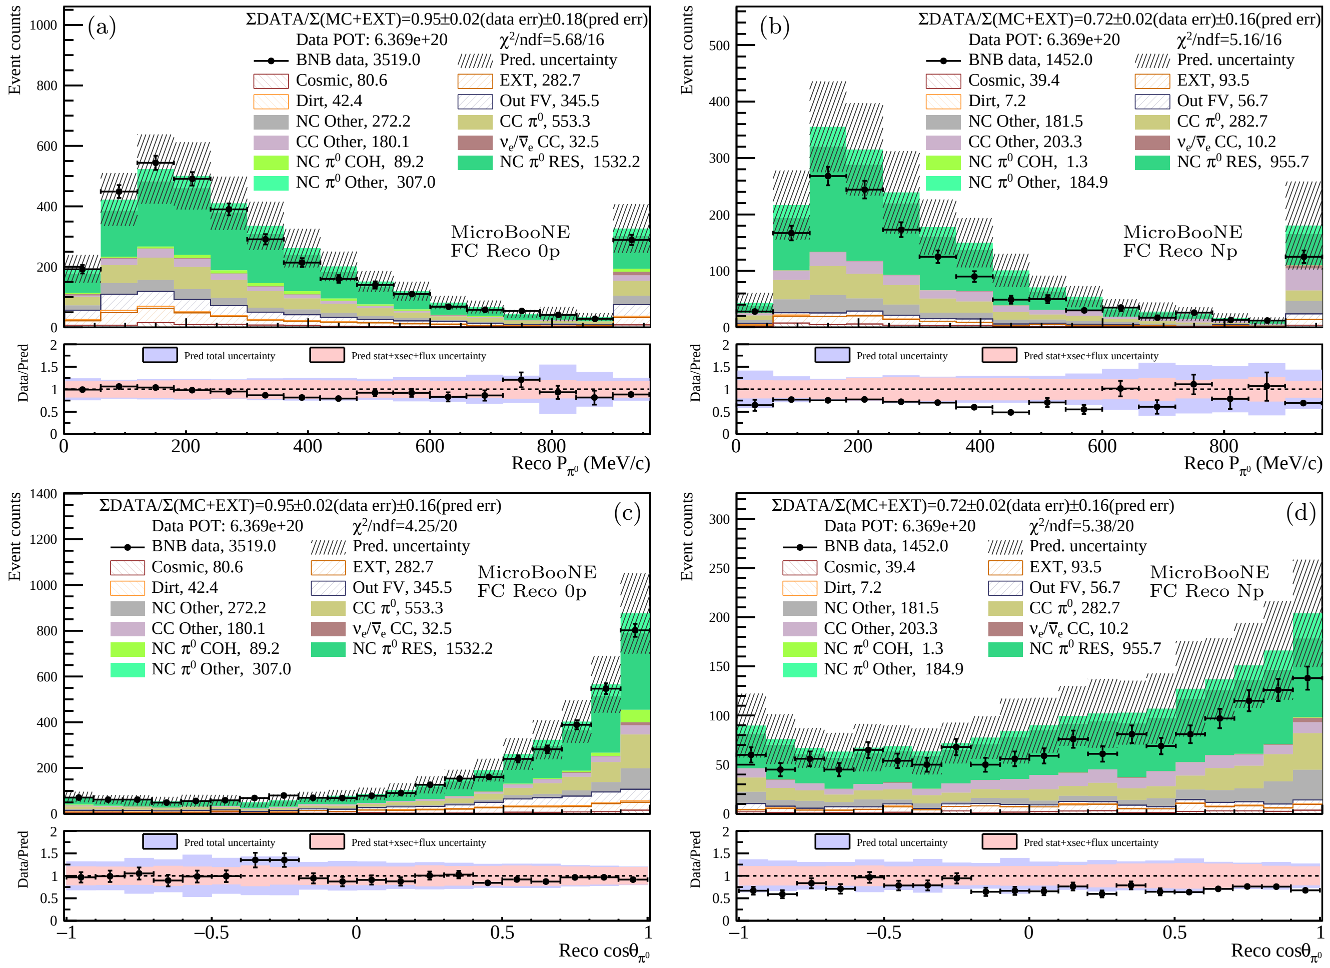


FIG. 21: Comparison between data and prediction for FC selected NC$\pi^0$ events as a function of reconstructed $\pi^0$ momentum [(a) and (b)] and the cosine of the reconstructed $\pi^0$ angle [(c) and (d)]. The reconstructed 0p selection is shown in (a) and (c), and the Np selection is shown in (b) and (d). In (a) and (b), the last bin corresponds to overflow. The statistical and systematic uncertainties of the prediction are shown in the bands. The data statistical errors are shown on the data points.

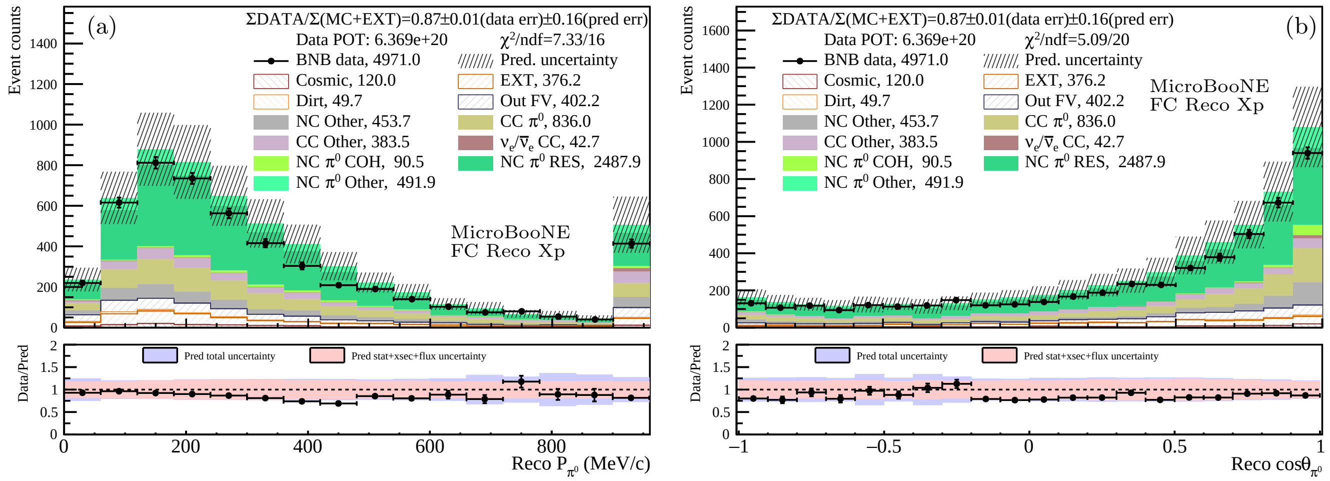


FIG. 22: Comparison between data and prediction for FC selected NC$\pi^0$ Xp events as a function of reconstructed $\pi^0$ momentum (a) and the cosine of the reconstructed $\pi^0$ angle (b). The last bin of (a) corresponds to overflow. The statistical and systematic uncertainties of the prediction are shown in the bands. The data statistical errors are shown on the data points.

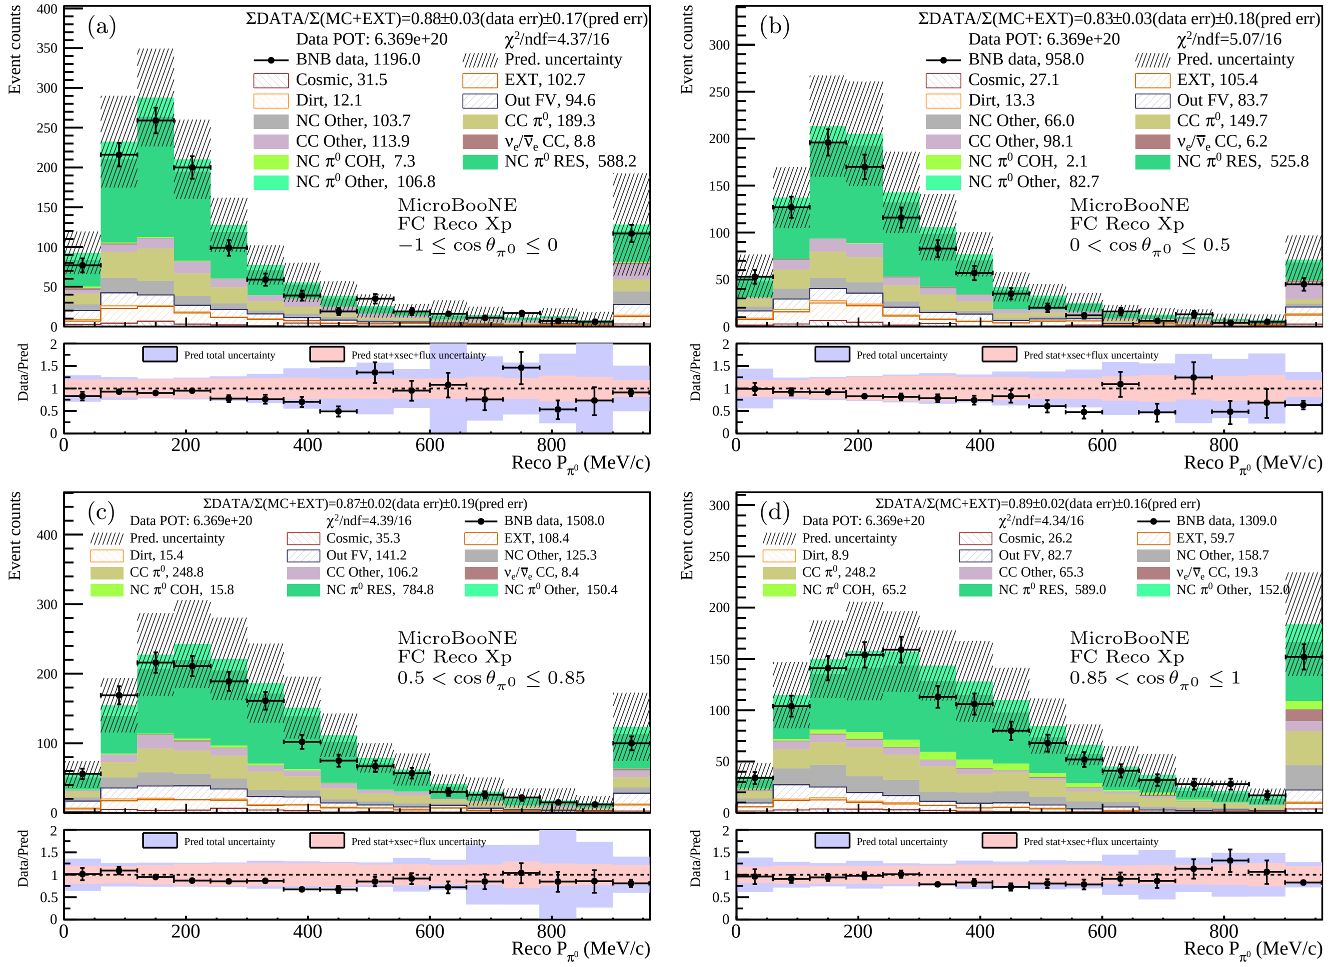


FIG. 23: Comparison between data and prediction as a function of reconstructed $\pi^0$ momentum for FC selected NC$\pi^0$ Xp events. Different $\cos\theta_{\pi^0}$ slices are shown in each subfigure. The last bin in each slice corresponds to overflow. The statistical and systematic uncertainties of the prediction are shown in the bands. The data statistical errors are shown on the data points.

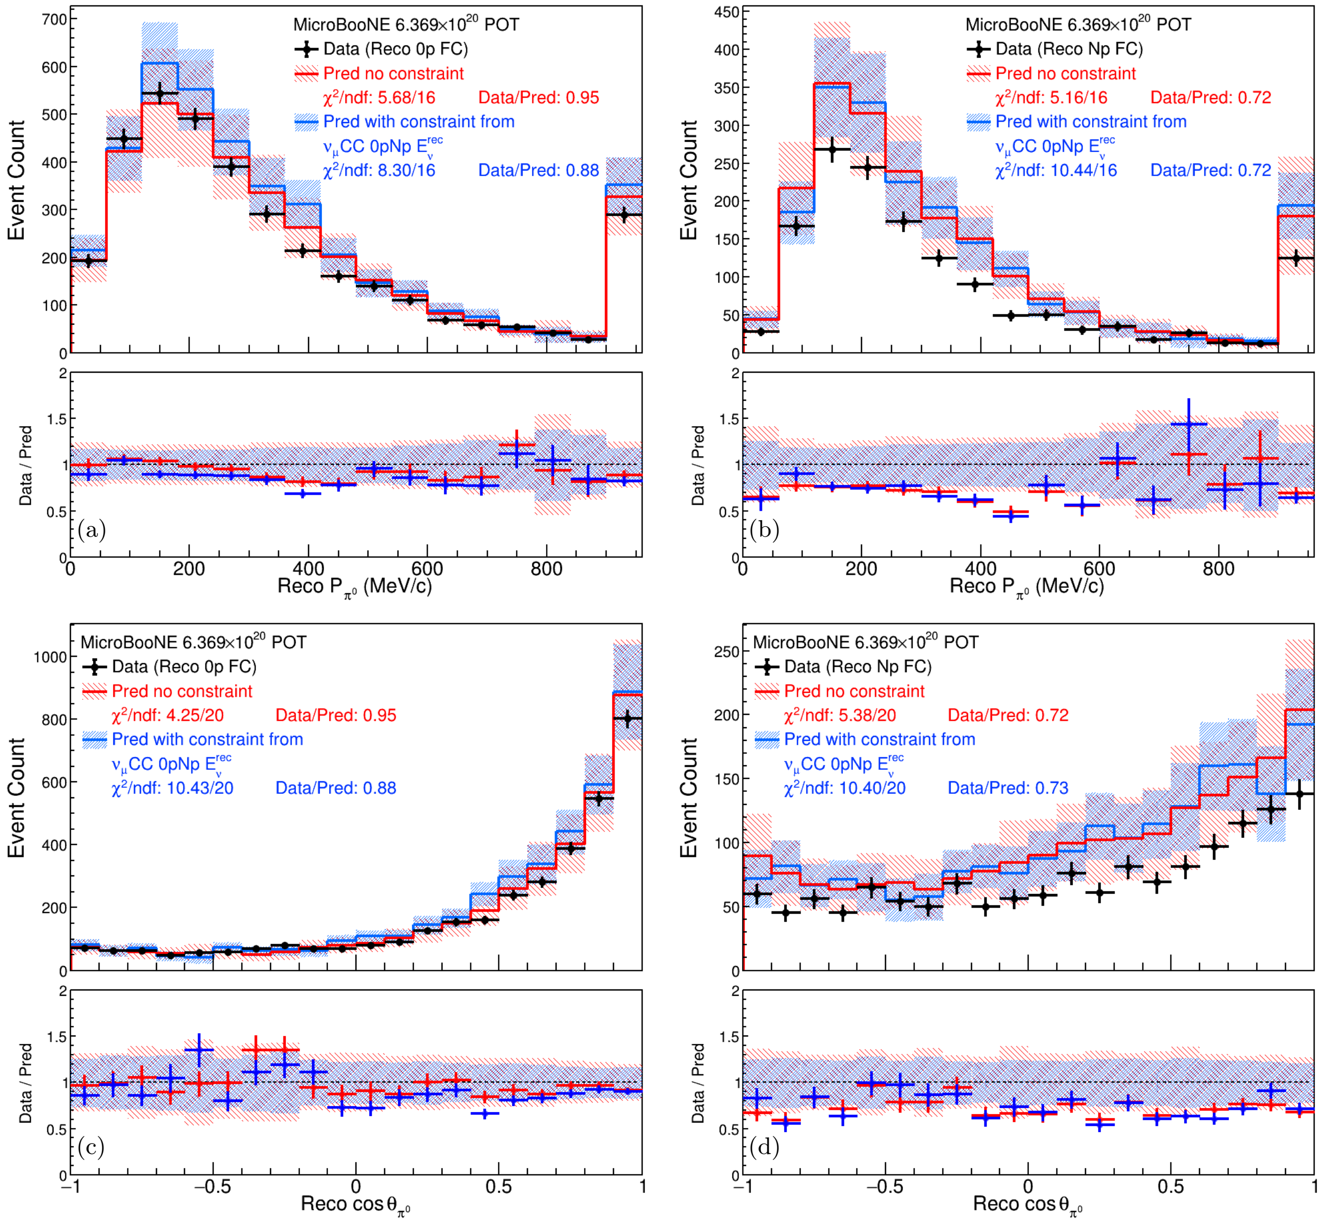


FIG. 24: Comparison between data and prediction for FC selected NC$\pi^0$ events as a function of reconstructed $\pi^0$ momentum [(a) and (b)] and the reconstructed $\pi^0$ angle [(c) and (d)]. The reconstructed 0p selection is shown in (a) and (c), the Np selection is shown in (b) and (d). In (a) and (b), the last bin corresponds to overflow. The red (blue) lines and bands show the prediction without (with) the constraint from the $\nu_\mu$CC reconstructed neutrino energy distribution. The statistical and systematic uncertainties of the prediction are shown in the bands. The data statistical errors are shown on the data points.

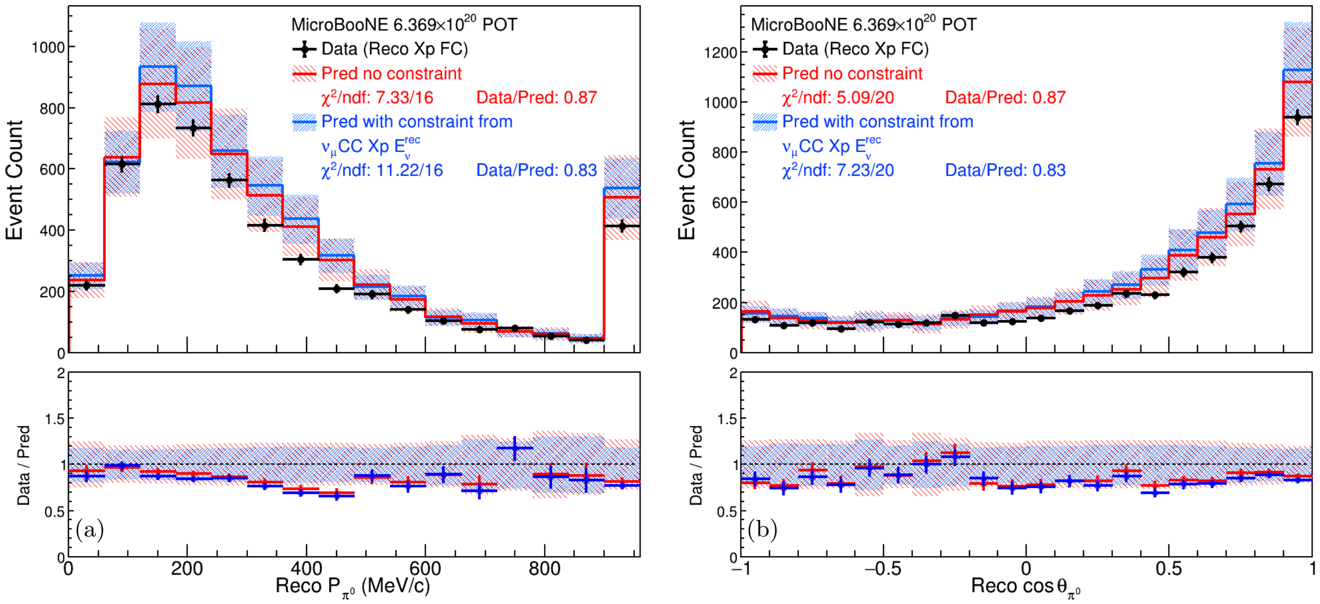


FIG. 25: Comparison between data and prediction for FC selected NC$\pi^0$ Xp events as a function of reconstructed $\pi^0$ momentum (a) and the reconstructed $\pi^0$ angle (b). In (a), the last bin corresponds to overflow. The red (blue) lines and bands show the prediction without (with) the constraint from the $\nu_\mu$CC reconstructed neutrino energy distribution. The statistical and systematic uncertainties of the prediction are shown in the bands. The data statistical errors are shown on the data points.

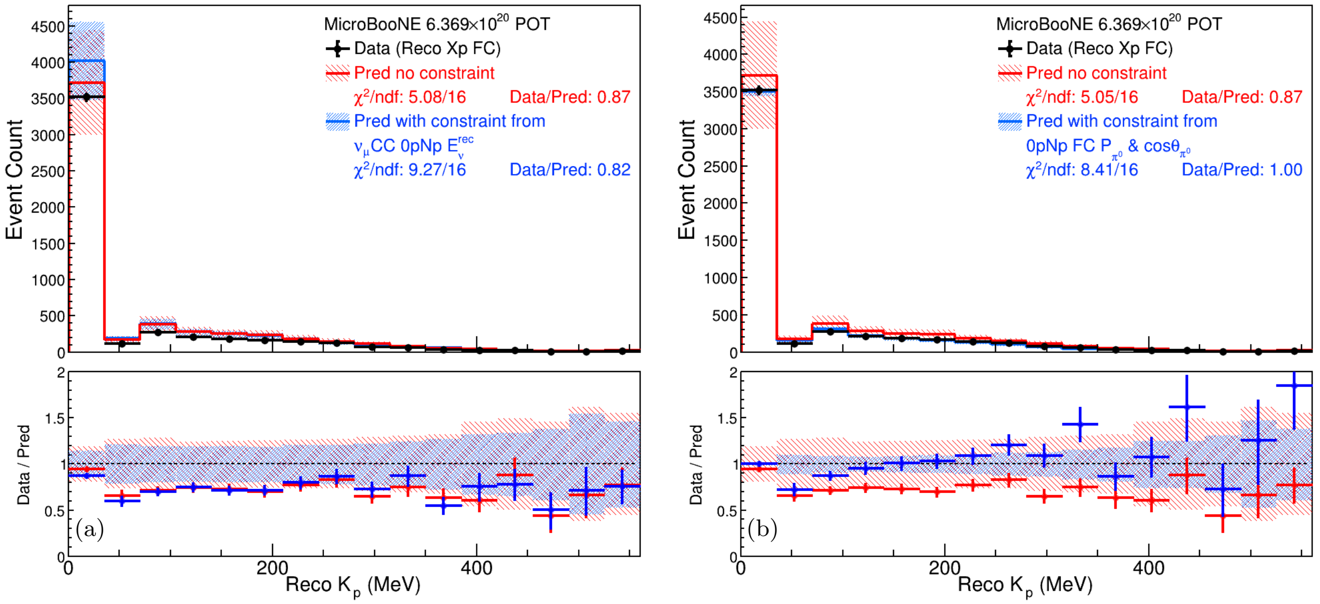


FIG. 26: Comparison between data and prediction as a function of reconstructed leading proton kinetic energy for FC selected NC$\pi^0$ events. The last bin corresponds to overflow. The red (blue) lines and bands show the prediction without (with) the constraint. In (a) the constraint is from the $\nu_\mu$CC reconstructed neutrino energy distribution and in (b) the constraint is from the the FC reconstructed $\pi^0$ momentum and angle distributions. The statistical and systematic uncertainties of the prediction are shown in the bands. The data statistical errors are shown on the data points.

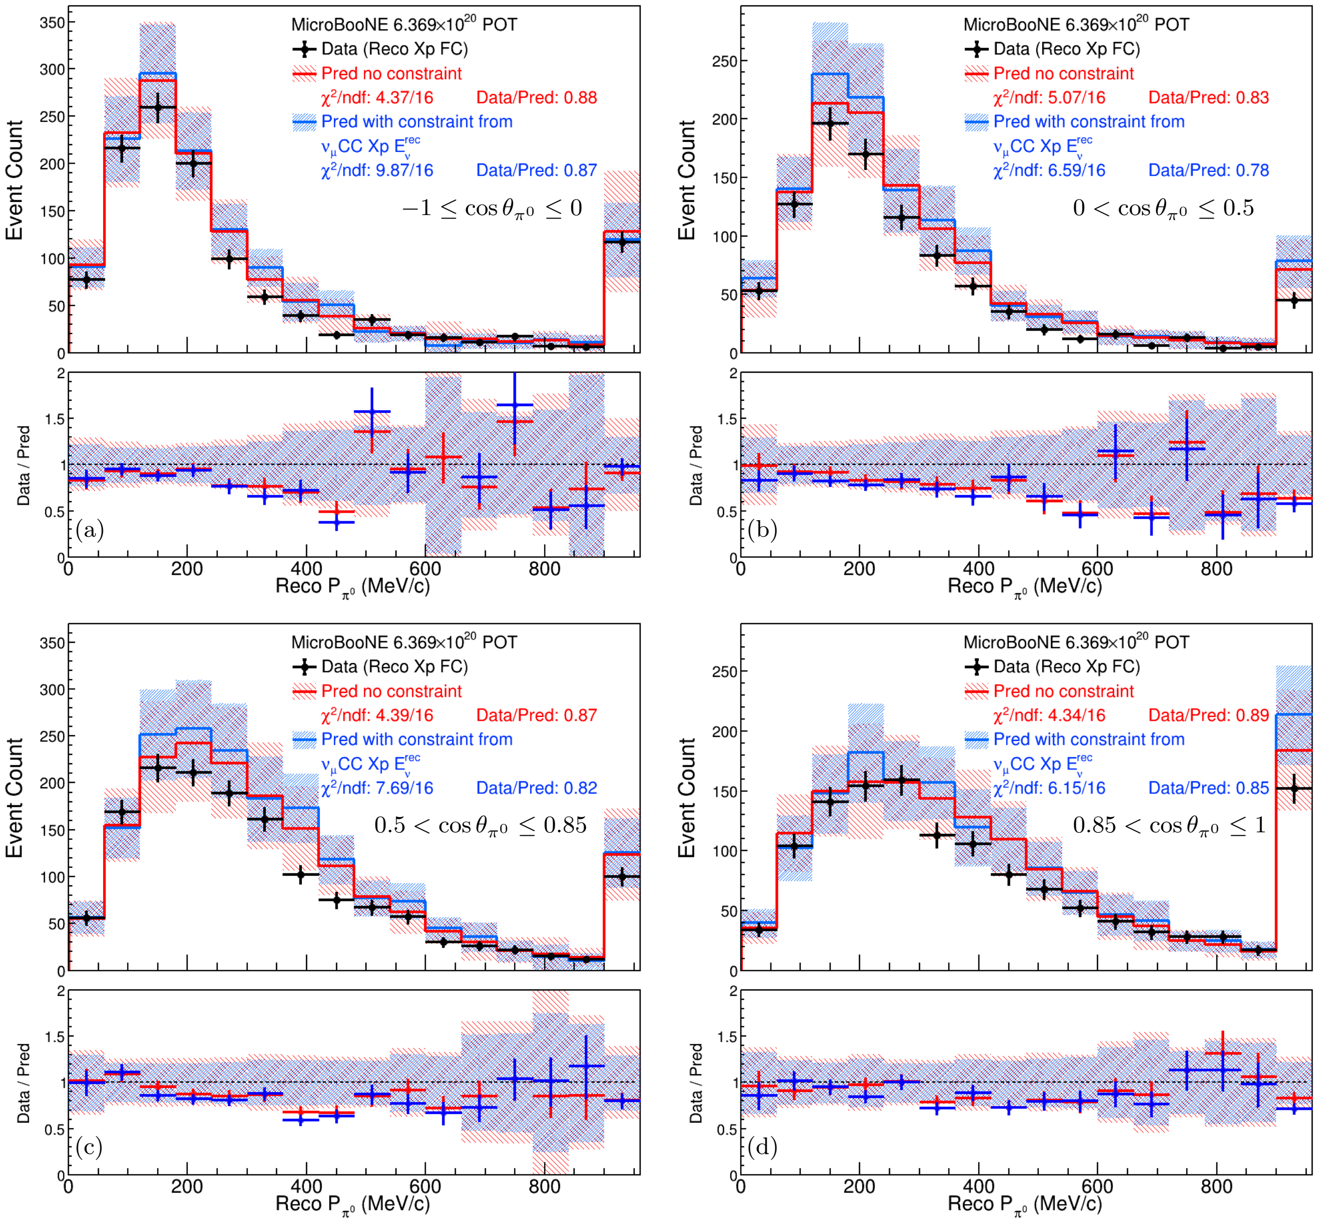


FIG. 27: Comparison between data and prediction as a function of reconstructed $\pi^0$ momentum for FC selected NC$\pi^0$ Xp events. Different $\cos\theta_{\pi^0}$ slices are shown in each subfigure. In all histograms, the last bin corresponds to overflow. The red (blue) lines and bands show the prediction without (with) the constraint from the $\nu_\mu$CC reconstructed neutrino energy distribution. The statistical and systematic uncertainties of the prediction are shown in the bands. The data statistical errors are shown on the data points. The $\chi^2/ndf$ across all bins after constraint is 27.0/64.

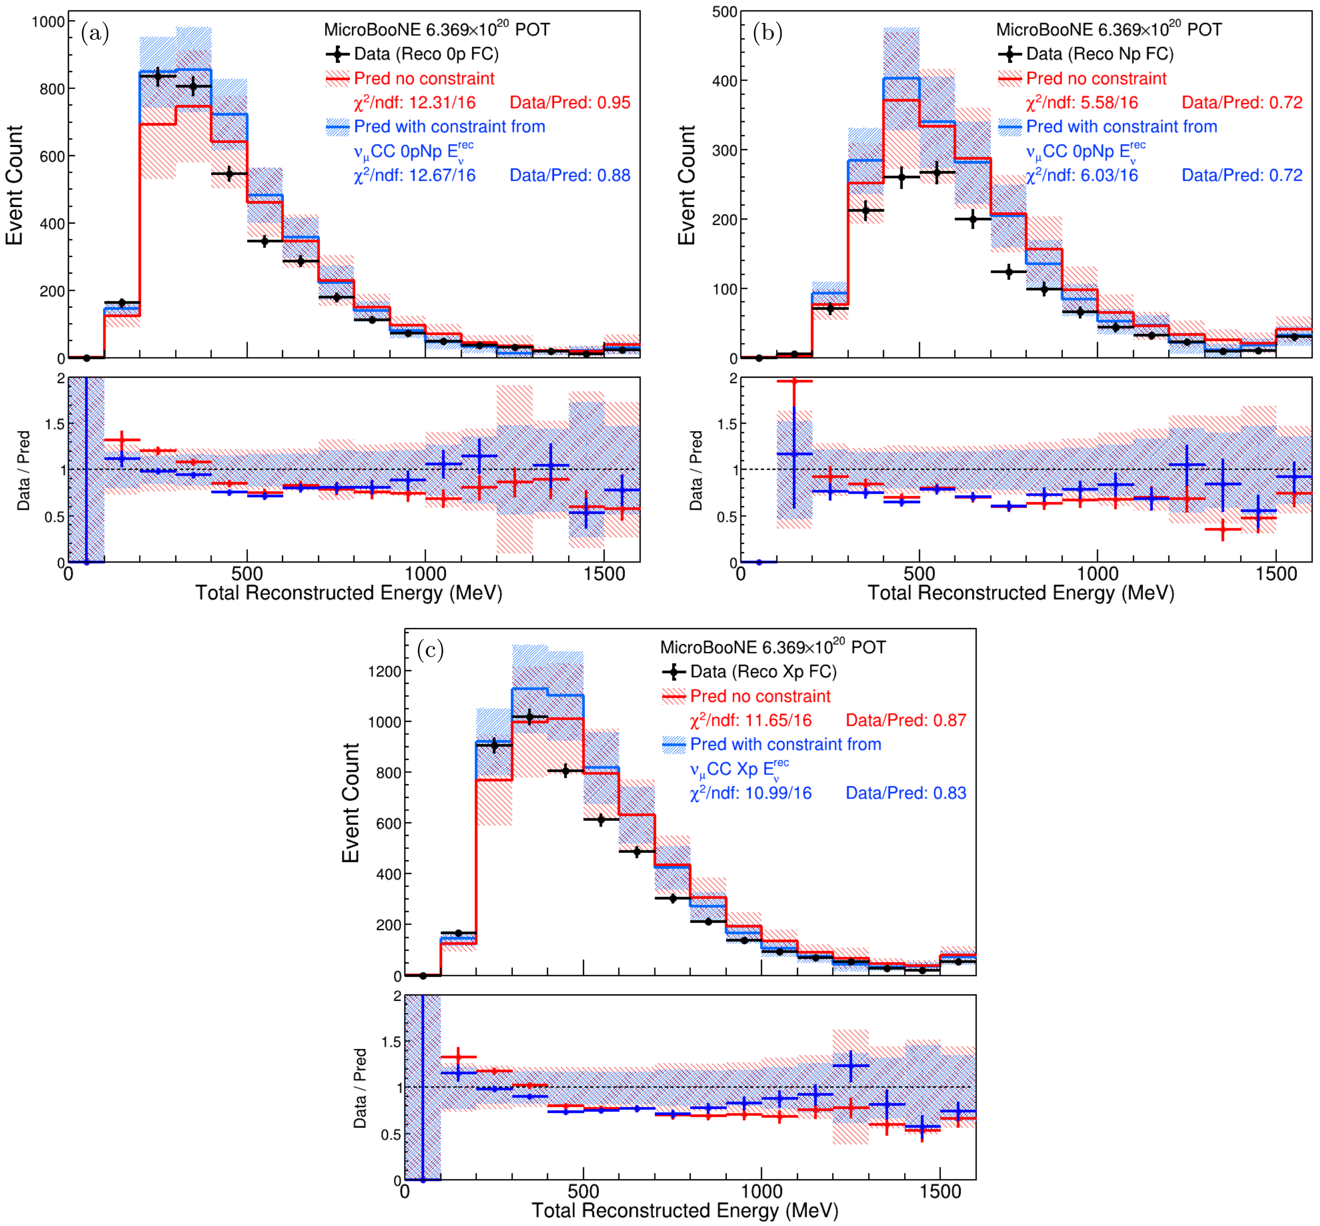


FIG. 28: Comparison between data and prediction as a function of the total reconstructed energy for FC selected NC$\pi^0$ events. The reconstructed 0p selection is shown in (a), the Np selection is shown in (b), and the Xp selection is shown in (c). The last bin corresponds to overflow in all histograms. The red (blue) lines and bands show the prediction without (with) the constraint from the $\nu_\mu$CC reconstructed neutrino energy distribution. The statistical and systematic uncertainties of the prediction are shown in the bands. The data statistical errors are shown on the data points.

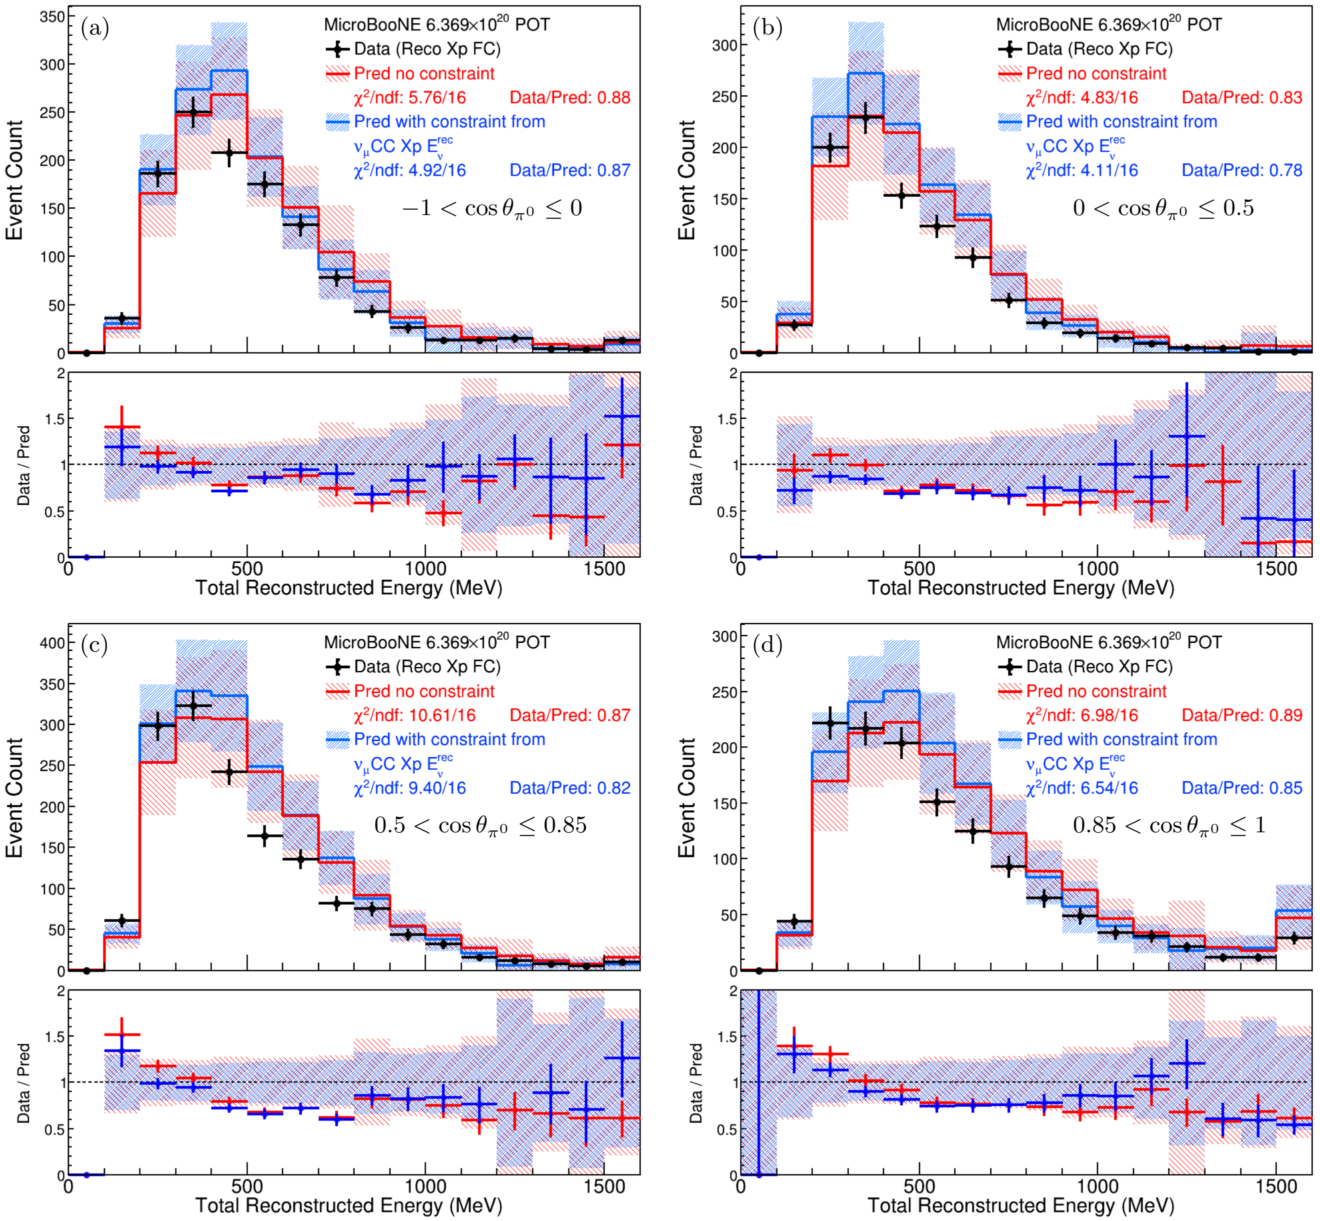


FIG. 29: Comparison between data and prediction as a function of the total reconstructed energy for FC selected NC$\pi^0$ Xp events. Different $\cos\theta_{\pi^0}$ slices are shown in each subfigure. In all histograms, the last bin corresponds to overflow. The red (blue) lines and bands show the prediction without (with) the constraint from the $\nu_\mu$CC reconstructed neutrino energy distribution. The statistical and systematic uncertainties of the prediction are shown in the bands. The data statistical errors are shown on the data points. The $\chi^2/ndf$ across all bins after constraint is 26.3/64.

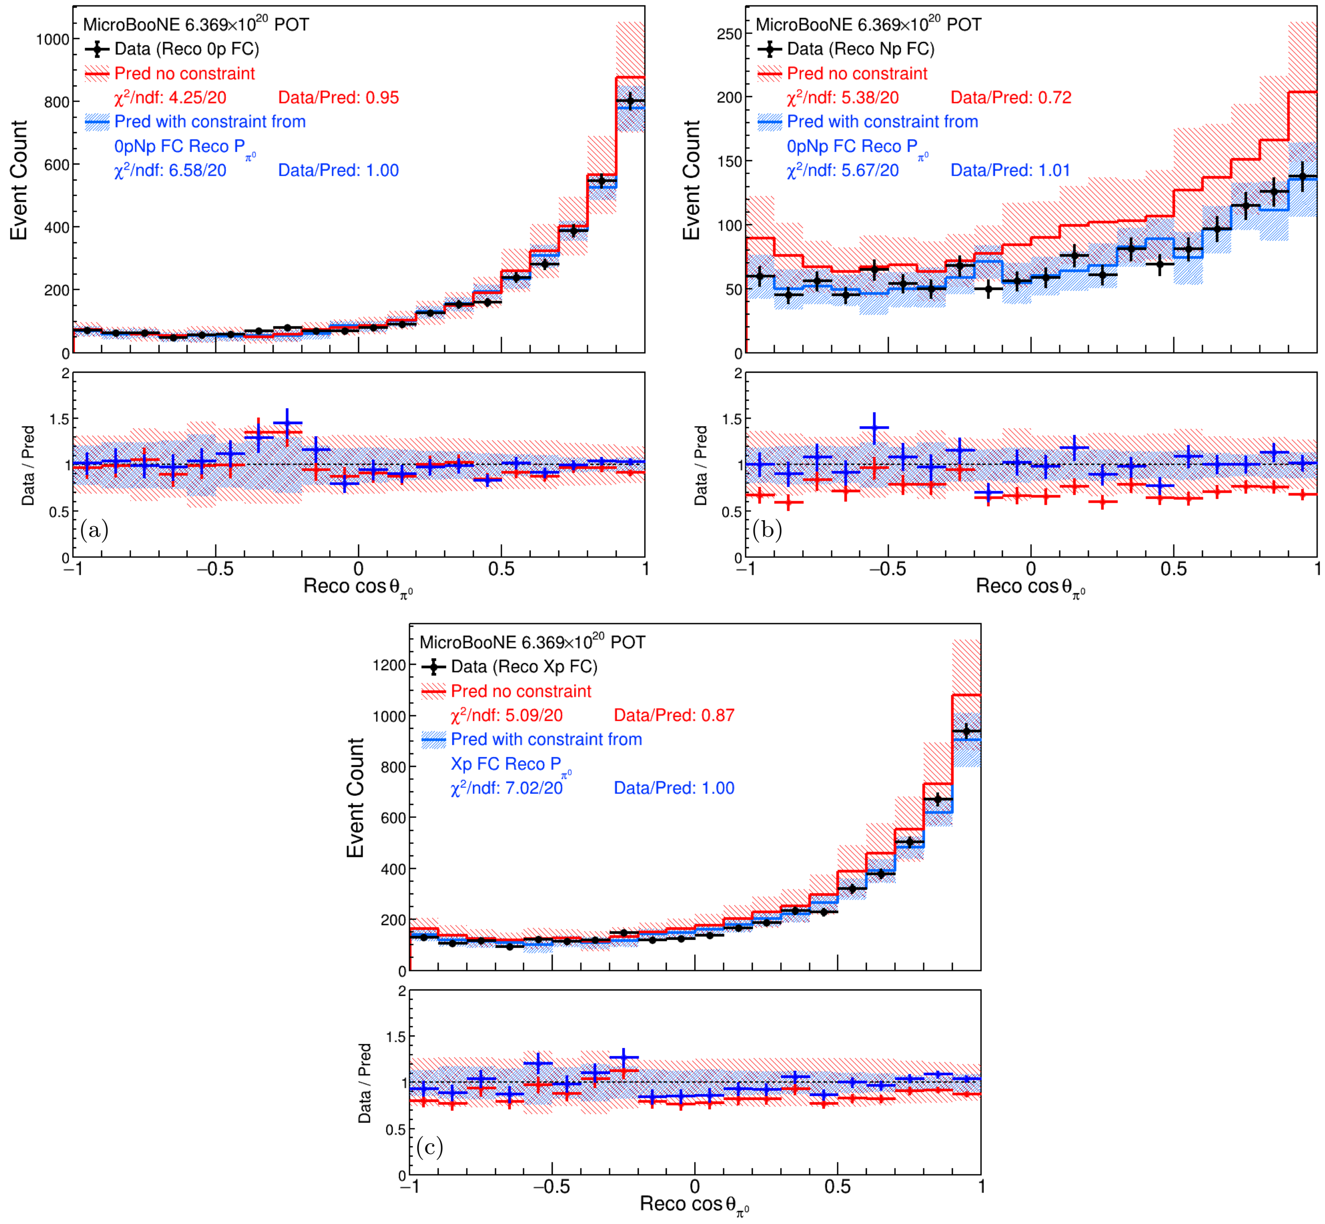


FIG. 30: Comparison between data and prediction as a function of the cosine of the reconstructed $\pi^0$ angle for FC selected NC$\pi^0$ events. The reconstructed 0p selection is shown in (a), the Np selection is shown in (b), and the Xp selection is shown in (c). The red (blue) lines and bands show the prediction without (with) the constraint from the FC reconstructed $\pi^0$ momentum distributions. The statistical and systematic uncertainties of the prediction are shown in the bands. The data statistical errors are shown on the data points.

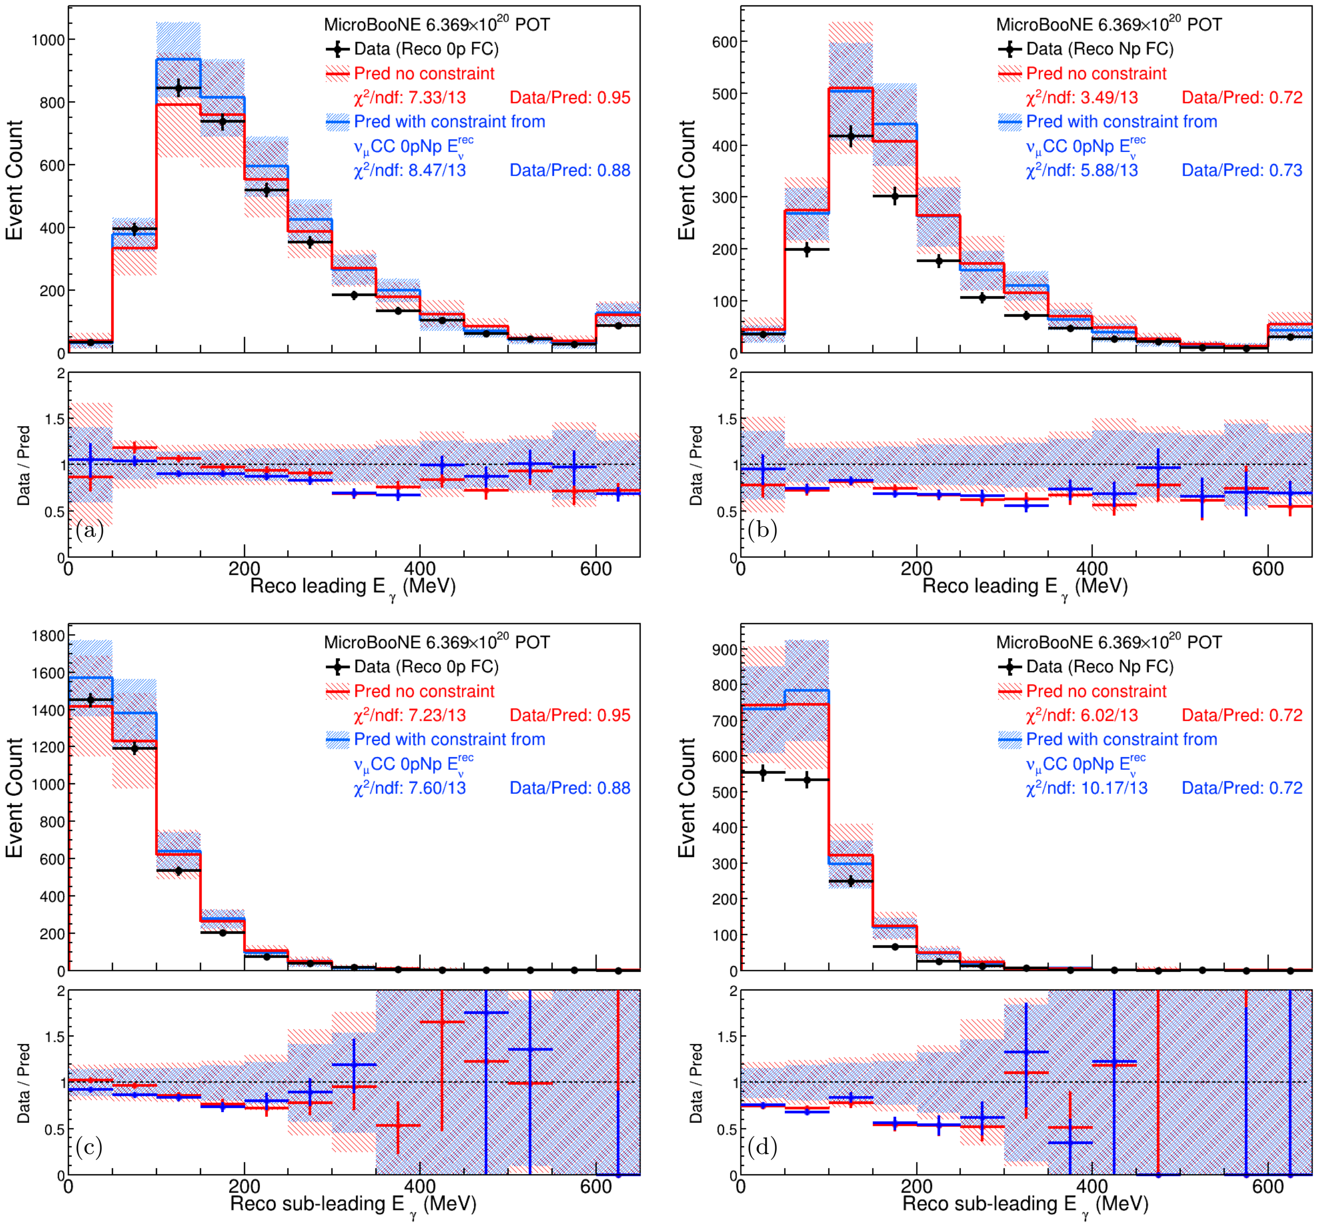


FIG. 31: Comparison between data and prediction for FC selected NC$\pi^0$ events as a function of reconstructed leading photon energy [(a) and (b)] and the reconstructed sub-leading photon energy. The reconstructed 0p selection is shown in (a) and (c), and the Np selection is shown in (b) and (d). The last bin corresponds to overflow in all histograms. The red (blue) lines and bands show the prediction without (with) the constraint from the $\nu_\mu$CC reconstructed neutrino energy distribution. The statistical and systematic uncertainties of the prediction are shown in the bands. The data statistical errors are shown on the data points.

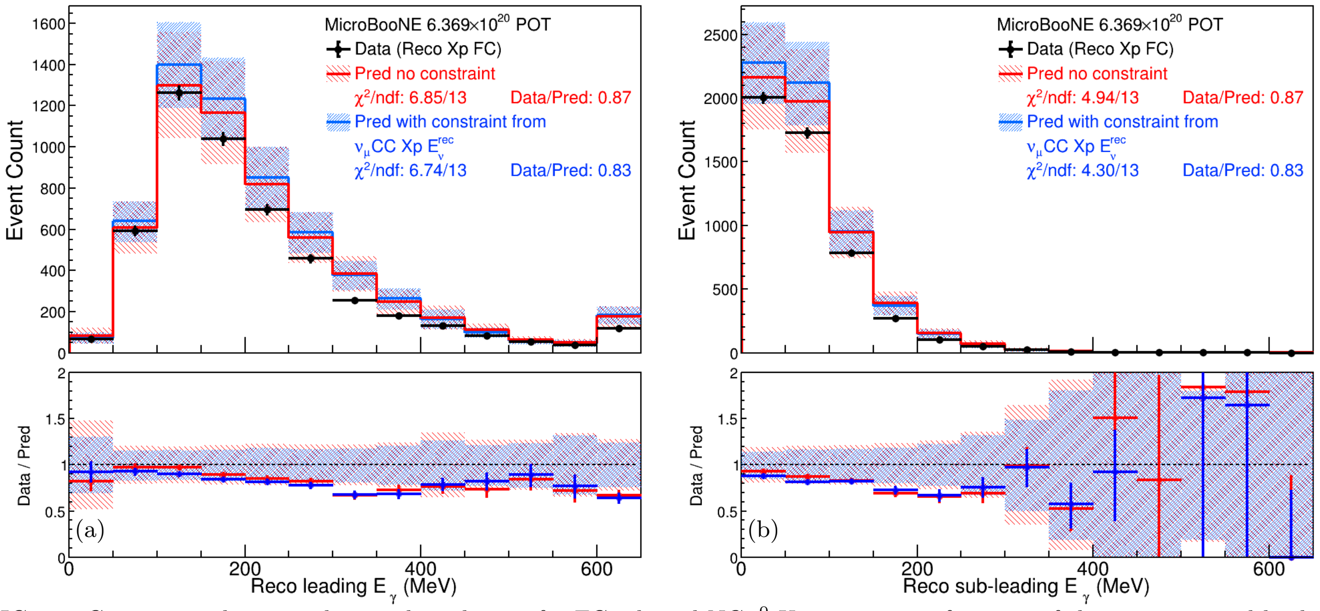


FIG. 32: Comparison between data and prediction for FC selected NC$\pi^0$ Xp events as a function of the reconstructed leading photon energy (a) and the reconstructed sub-leading photon energy (b). The last bin corresponds to overflow in all histograms. The red (blue) lines and bands show the prediction without (with) the constraint from the $\nu_\mu$CC reconstructed neutrino energy distribution. The statistical and systematic uncertainties of the prediction are shown in the bands. The data statistical errors are shown on the data points.

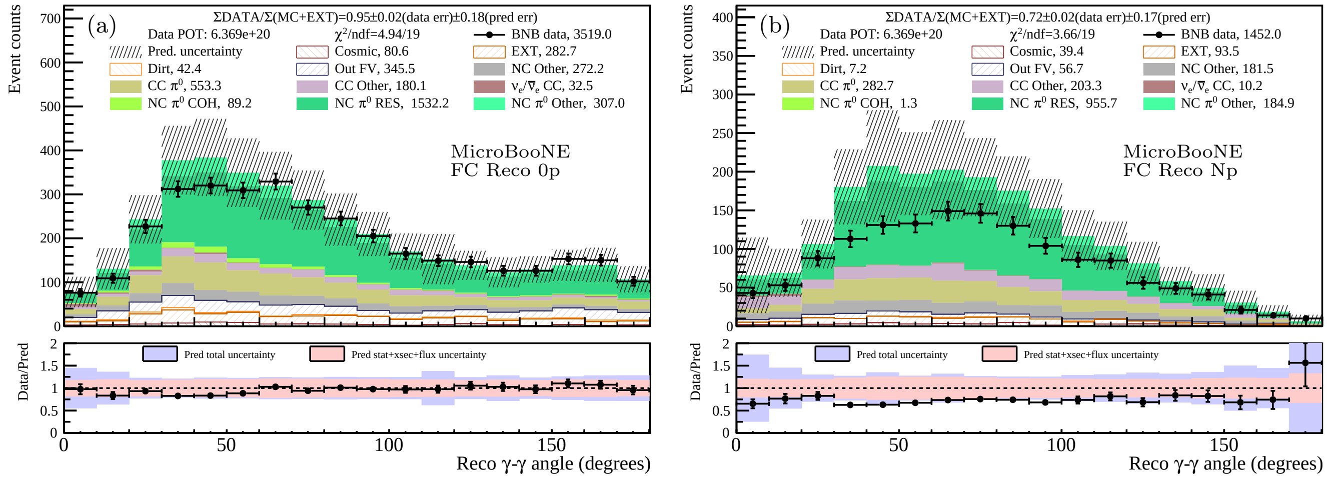


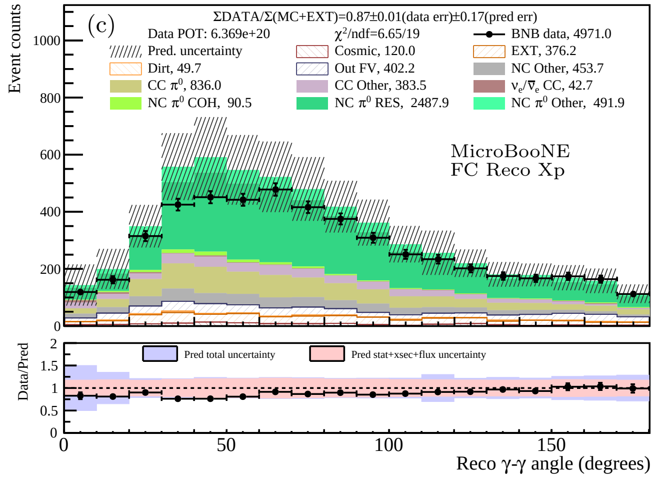


FIG. 33: Comparison between data and prediction as a function of reconstructed angle between the $\pi^0$ decay photons for FC selected NC$\pi^0$ events. The reconstructed 0p selection is shown in (a), the Np selection is shown in (b), and the Xp selection is shown in (c). The statistical and systematic uncertainties of the prediction are shown in the bands. The data statistical errors are shown on the data points.

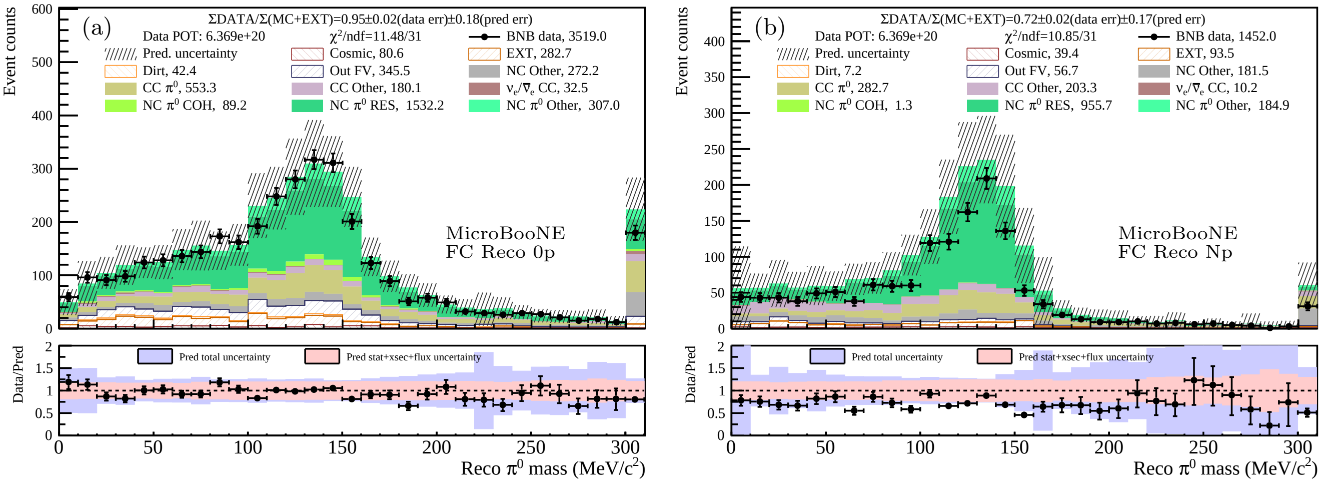


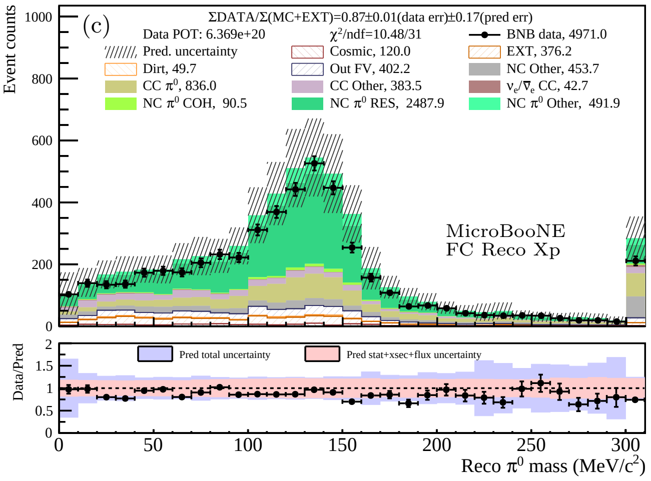


FIG. 34: Comparison between data and prediction as a function of reconstructed invariant mass for FC selected NC$\pi^0$ events. The reconstructed 0p selection is shown in (a), the Np selection is shown in (b), and the Xp selection is shown in (c). The last bin corresponds to overflow in all histograms. The statistical and systematic uncertainties of the prediction are shown in the bands. The data statistical errors are shown on the data points.

## VI. FAKE DATA STUDIES

Fake data studies were carried out to test the robustness of the model validation and cross section extraction. For the studies presented here, a `NuWro 19.02.2` MC sample was propagated thought the MicroBooNE simulation and reconstruction chain in the same way as the nominal `GENIEv3`-based $\mu$`BooNE` tune MC, after which it was treated identically to real data. Because the fake data and MC prediction use the same detector and flux simulations, uncertainties due to beam exposure, number of targets, detector, fluxes, and reinteractions are fully correlated and not included. Only the uncorrelated uncertainties (cross section, statistical, and MC statistical) are used for the model validation, the cross section extraction, and the subsequent $\chi^2$ calculations between the fake data results and generator predictions.

The same model validation used for real data was applied to the fake data. These tests expose some disagreement between the `NuWro` fake data and MC predictions, indicating that the model does not necessarily have sufficient uncertainties to extract fake data cross section without inducing bias. In particular, tests on the distribution of the reconstructed proton kinetic energy, $K_p^{rec}$, and the total reconstructed energy in backwards $\pi^0$ angular slices yield $p$-values of 0.02 and 0.11, respectively. This level of tension that would either fail validation, or comes close enough to failing that further investigation would be warranted. These test can be seen in Fig. 35. If this scenario were encountered in real data, the tension would be mitigated by an updated model prediction or an expanded uncertainty budget through a procedure analogous to that of [2]. Furthermore, the Np $\cos\theta_{\pi^0}^{rec}$ distribution shows a significant deficit in the most forward bin which is not mitigated by the constraint from the $\nu_\mu$CC reconstructed neutrino energy distribution nor the $P_{\pi^0}^{reco}$ distribution. This distribution can be seen in Fig. 36. This is possibly related to the failure of the model validation for $K_p^{rec}$, which indicates significant differences with respect to the modeling of the final state proton kinetic energy and the division into 0p and Np final states. For real data, seeing such a large deficit that was worsened, rather than improved, by the constraints would likewise motivate further investigation before the model was considered validated.

Despite the moderate tension seen in the model validation, cross section results were subsequently extracted for

all intended measurements without an expansion to the nominal model used for unfolding. The results can be seen throughout the rest of this section. Note that the 0p and Np cross sections were extracted simultaneously; the formulation for such an extraction is described in more detail in [2]. Subsequent figures contain the extracted fake data differential cross section as well as predictions from `NuWro 19.02.2` (`NuWro 19`), `NuWro 21.02` (`NuWro`), `GENIE v2.12.10` (`GENIEv2`), `GENIE v3.0.6 G18_10a_02_11a` (`GENIEv3`) [7], `NEUT 5.4.0.1` (`NEUT`) [8], and `GiBUU 2023` (`GiBUU`). These include predictions using the default generator parameters and the predictions included in the main text and Sec. VII of the Supplemental Material that modify the form factors describing the neutrino-nucleon interaction, the FSI experienced by the outgoing particles, and the contribution from coherent scattering. These generator predictions were processed with the `NUISANCE` framework [9], and each has been smeared with the $A_C$ matrix obtained from unfolding the fake data.

Closure of the study is achieved when the fake data shows good agreement with the `NuWro 19` prediction (blue line). This is quantified by the $\chi^2/ndf$ calculated between the fake data and prediction with uncertainties according to the extracted covariance matrix. The `NuWro 19` prediction was generated independently and at higher stats than the fake data, which, at $6.11 \times 10^{20}$ POT, is comparable in size to the real data set. Despite the tension seen in the model validation, acceptable closure is achieved in all cases, with $\chi^2/ndf$ values around or below unity. The extracted fake data cross sections agree with the `NuWro 19` prediction approximately as well as, or better than, they do with any other generator. The `NuWro 19` prediction also falls within $1\sigma$ of the extracted results on almost all bins. The Np $\cos\theta_{\pi^0}$ result does show some bias towards lower values in the most forward bins, which is unsurprising given the results of the model validation, as the Wiener-SVD unfolding smears the observed deficit in the most forward $\cos\theta_{\pi^0}^{rec}$ bin across the the first several bins during the extraction. Nevertheless, the resulting $\chi^2$ calculated for the Np $\cos\theta_{\pi^0}$ result and `NuWro 19` prediction still indicates good agreement and a successful cross section extraction. The situation is similar for the double-differential fake data result. Though showing some bias on a bin-by-bin basis around the peak of the distribution in the two more forward angular slices, this fake data result shows reasonable closure in terms of $\chi^2$ values, which properly considers the correlations between bins that are not visually obvious. This is true both on individual angular slices and on the distribution as a whole, again indicating a relatively successfully cross section extraction despite the tension identified in the model validation. These tests of the unfolding give us confidence that the model validation is sufficient for detecting potentially relevant mismodeling and that the cross section extraction methodology is reasonably robust even in cases where moderate tension is seen in the validation.

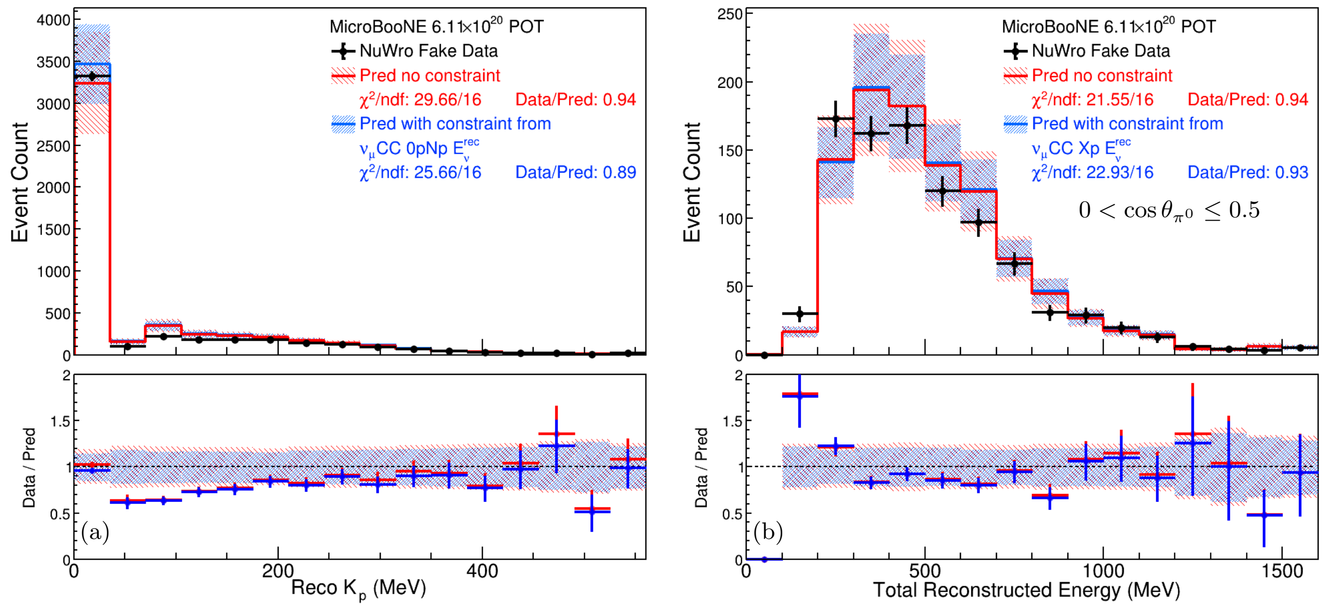


FIG. 35: Results of several model validation tests for `NuWro` fake data study that either fail, or nearly fail model validation. The comparison between the `NuWro` fake data and model prediction for FC selected NC$\pi^0$ Xp events as a function of reconstructed leading proton kinetic energy is shown in (a), and the comparison between `NuWro` fake data and model prediction for FC selected NC$\pi^0$ Xp events with $0 \leq \cos\theta_{\pi^0} \leq 0.5$ as a function of $P_{\pi^0}^{reco}$ is shown in (b). The last bin corresponds to overflow in all histograms. The red (blue) lines and bands show the prediction without (with) constraint from the $\nu_\mu$CC reconstructed neutrino energy distribution. The statistical and systematic uncertainties of the prediction are shown in the bands. The data statistical errors are shown on the data points.

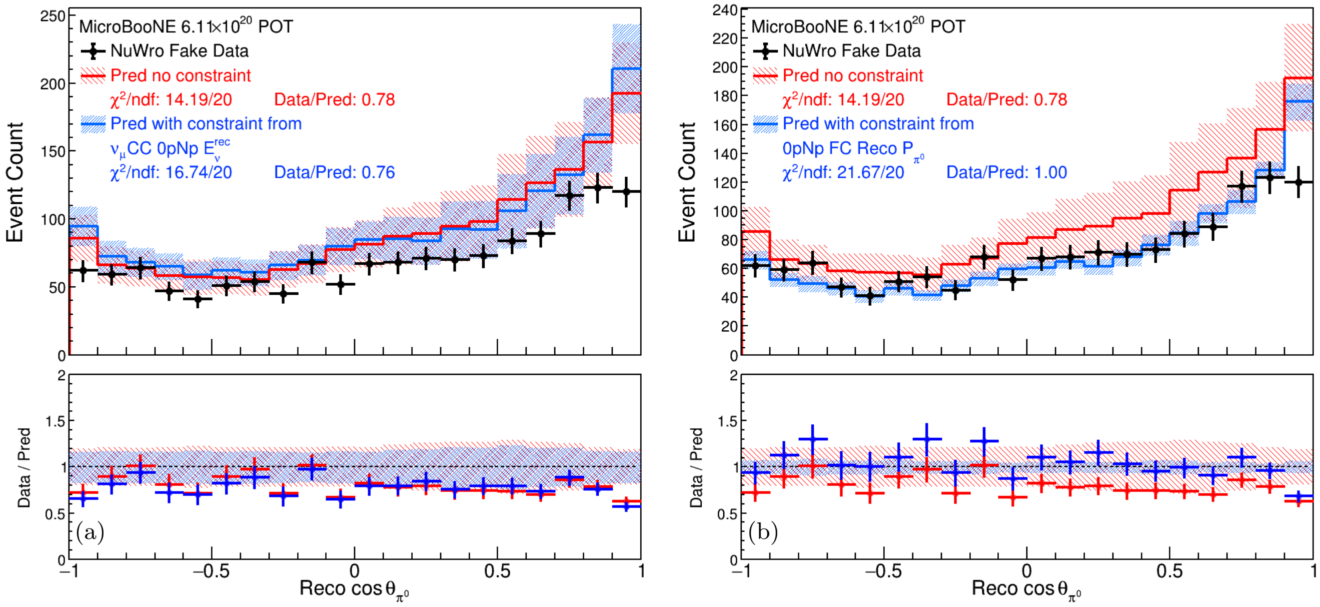


FIG. 36: Comparison between `NuWro` fake data and model prediction for FC selected NC$\pi^0$ Np events with as a function of $cos\theta_{\pi^0}^{rec}$. The red (blue) lines and bands show the prediction without (with) the constraint. The $\nu_\mu$CC reconstructed neutrino energy distribution is used for the constraint in (a) and the $P_{\pi^0}^{reco}$ distribution is used in (b). The statistical and systematic uncertainties of the prediction are shown in the bands. The data statistical errors are shown on the data points.

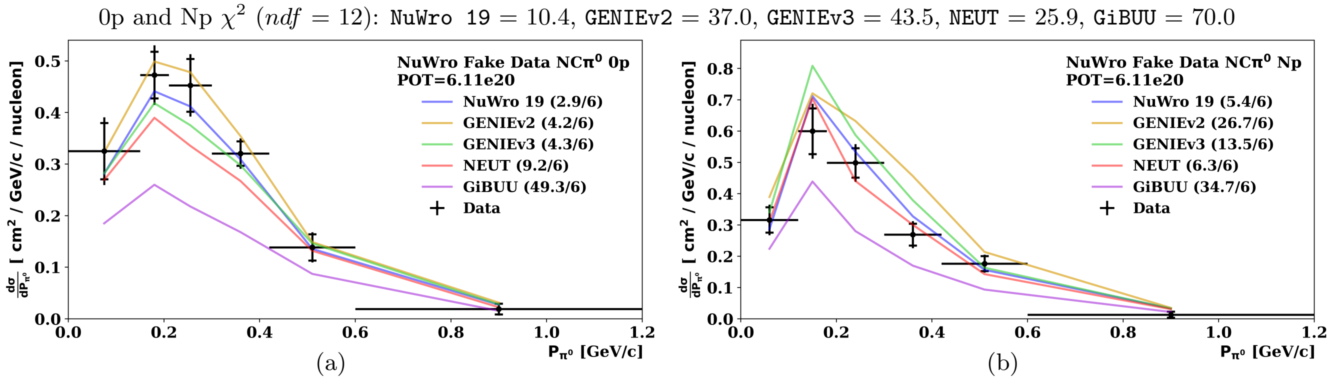


FIG. 37: Unfolded `NuWro 19` fake data 0p and Np $P_{\pi^0}$ differential cross section results. The 0p result is shown in (a) and the Np result is shown in (b). The black inner (outer) error bars on the data points represent the statistical (total) uncertainties on the extracted cross section corresponding to the square root of the diagonal elements of the extracted covariance matrix. Different generator predictions are indicated by the colored lines with corresponding $\chi^2$ values displayed in the legend. The $\chi^2$ values calculated using all bins are shown at the top of the figure.

0p and Np $\chi^2$ ($ndf$ = 23): NuWro = 21.5, GENIEv2 = 40.3, GENIEv3 = 53.6, NEUT = 36.7, GiBUU = 77.1

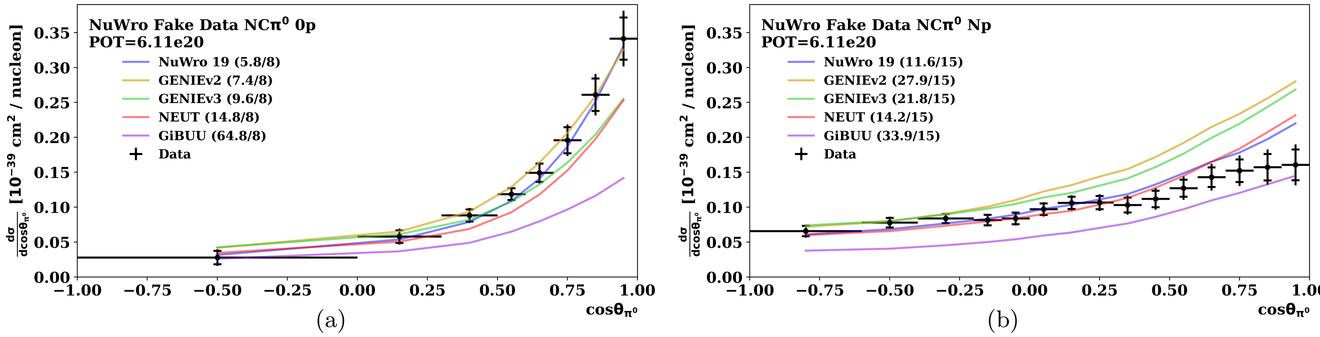


(a) (b)

FIG. 38: Unfolded NuWro 19 fake data 0p and Np $\cos\theta_{\pi^0}$ differential cross section results. The 0p result is shown in (a) and the Np result is shown in (b). The black inner (outer) error bars on the data points represent the statistical (total) uncertainties on the extracted cross section corresponding to the square root of the diagonal elements of the extracted covariance matrix. Different generator predictions are indicated by the colored lines with corresponding $\chi^2$ values displayed in the legend. The $\chi^2$ values calculated using all bins are shown at the top of the figure.

$\chi^2$ for all bins ($ndf$ = 24): NuWro 19 = 25.0, GENIEv2 = 37.8, GENIEv3 = 20.7, NEUT = 26.2, GiBUU = 91.0

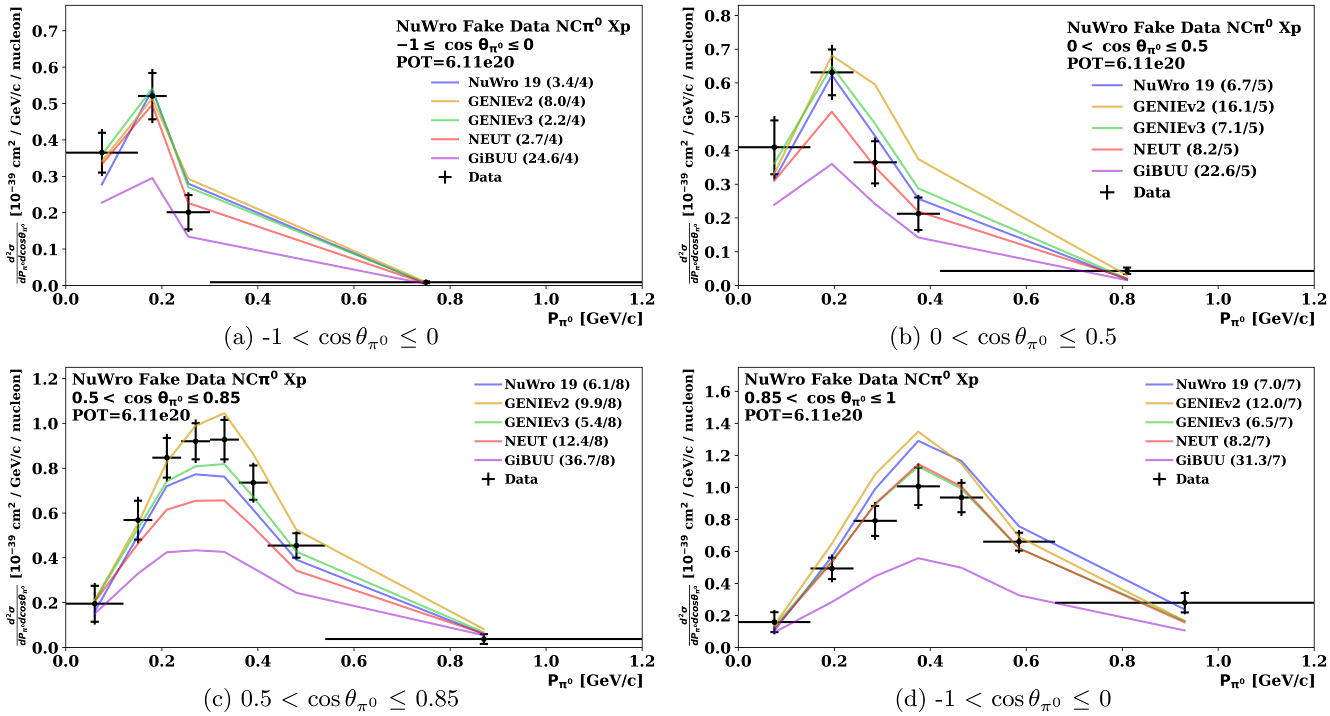


(a) -1 < $\cos\theta_{\pi^0}$ ≤ 0 (b) 0 < $\cos\theta_{\pi^0}$ ≤ 0.5

(c) 0.5 < $\cos\theta_{\pi^0}$ ≤ 0.85 (d) -1 < $\cos\theta_{\pi^0}$ ≤ 0

FIG. 39: Unfolded NuWro 19 fake data Xp $\cos\theta_{\pi^0}$ and $P_{\pi^0}$ double-differential cross section result. The black inner (outer) error bars on the data points represent the statistical (total) uncertainties on the extracted cross section corresponding to the square root of the diagonal elements of the extracted covariance matrix. Different generator predictions are indicated by the colored lines with corresponding $\chi^2$ values calculated for the given slice displayed in the legend. The $\chi^2$ values calculated using all bins are shown at the top of the figure.

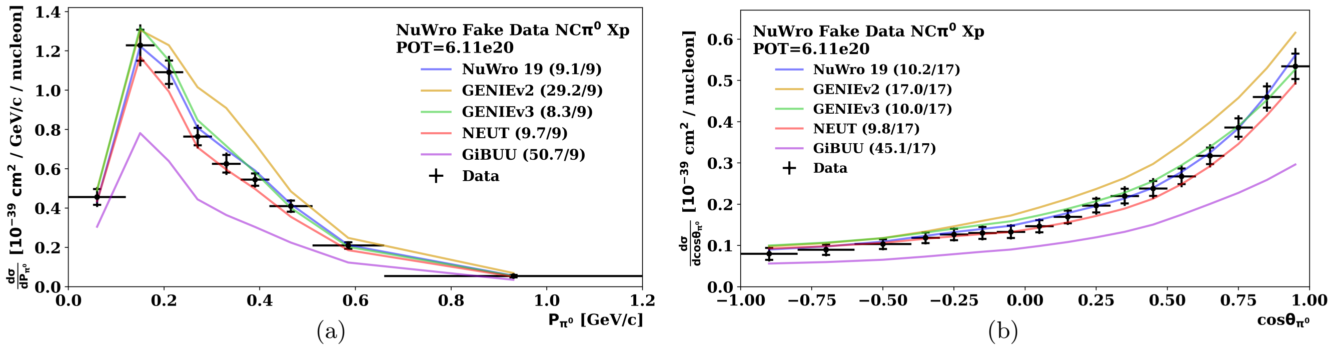


FIG. 40: Unfolded `NuWro 19` fake data Xp $P_{\pi^0}$ differential cross section result (a) and Xp $\cos\theta_{\pi^0}$ differential cross section result (b). The black inner (outer) error bars on the data points represent the statistical (total) uncertainties on the extracted cross section corresponding to the square root of the diagonal elements of the extracted covariance matrix. Different generator predictions are indicated by the colored lines with corresponding $\chi^2$ values displayed in the legend.

0p and Np $\chi^2$ ($ndf = 12$): `NuWro 19 (no FSI)` = 10.4 (132.5), `GENIEv3 (no FSI)` = 43.5 (197.1), `NEUT (no FSI)` = 25.9 (148.7), `GiBUU (no FSI)` = 70.0 (115.6)

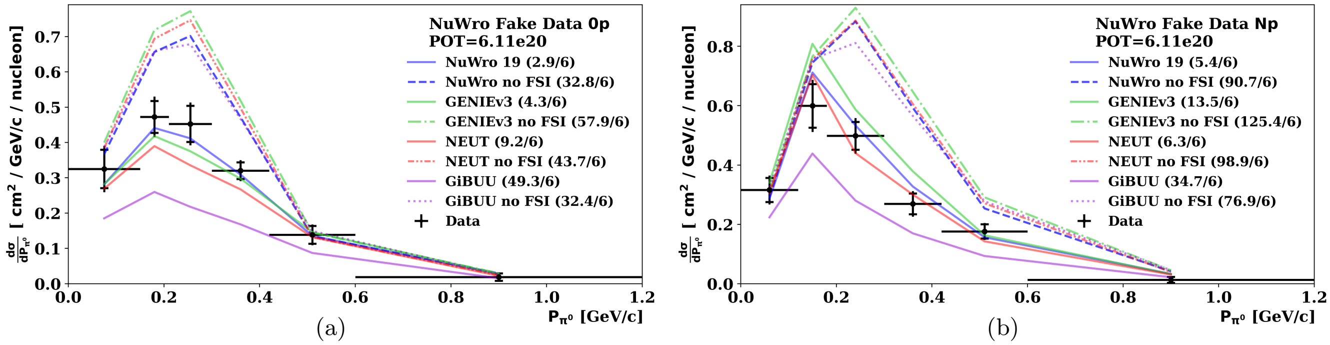


FIG. 41: Same as Fig. 37, but with the generator predictions from Fig. 1 of the main text that modify the FSI.

0p and Np $\chi^2$ ($ndf = 23$): `NuWro 19` = 21.5, `GENIEv3` = 53.6, `GENIEv3 no COH` = 59.1, `NEUT` = 36.7, `NEUT no COH` = 50.9, `GiBUU` = 77.1, `GiBUU wi NEUT COH` = 55.1

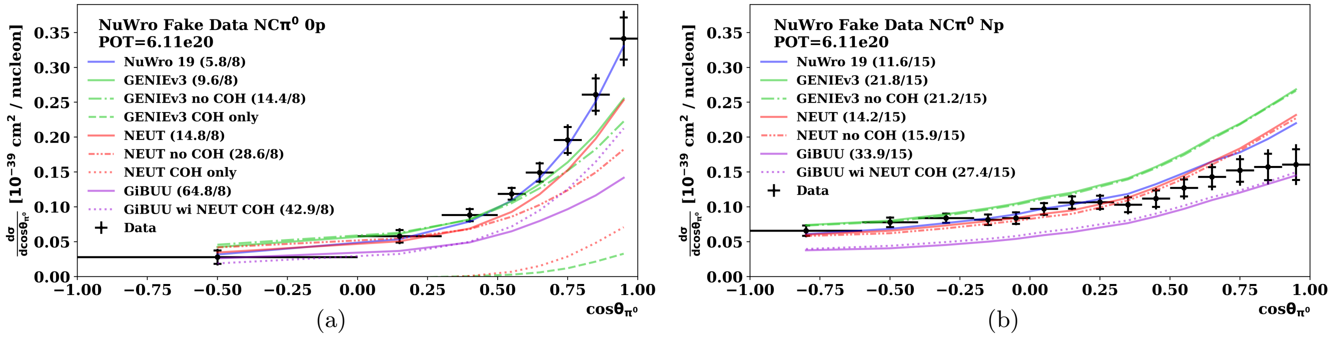


FIG. 42: Same as Fig. 38, but with the generator predictions from Sec. VII that modify coherent pion production.

$\chi^2$ for all bins ($ndf$ = 24): NuWro 19 = 25.0, NuWro = 29.7, NuWro FF1 ($M_A$=1.05) = 28.1, NuWro FF1 ($M_A$=0.84) = 36.7, NuWro FF2 = 41.0, NuWro FF3 = 32.9

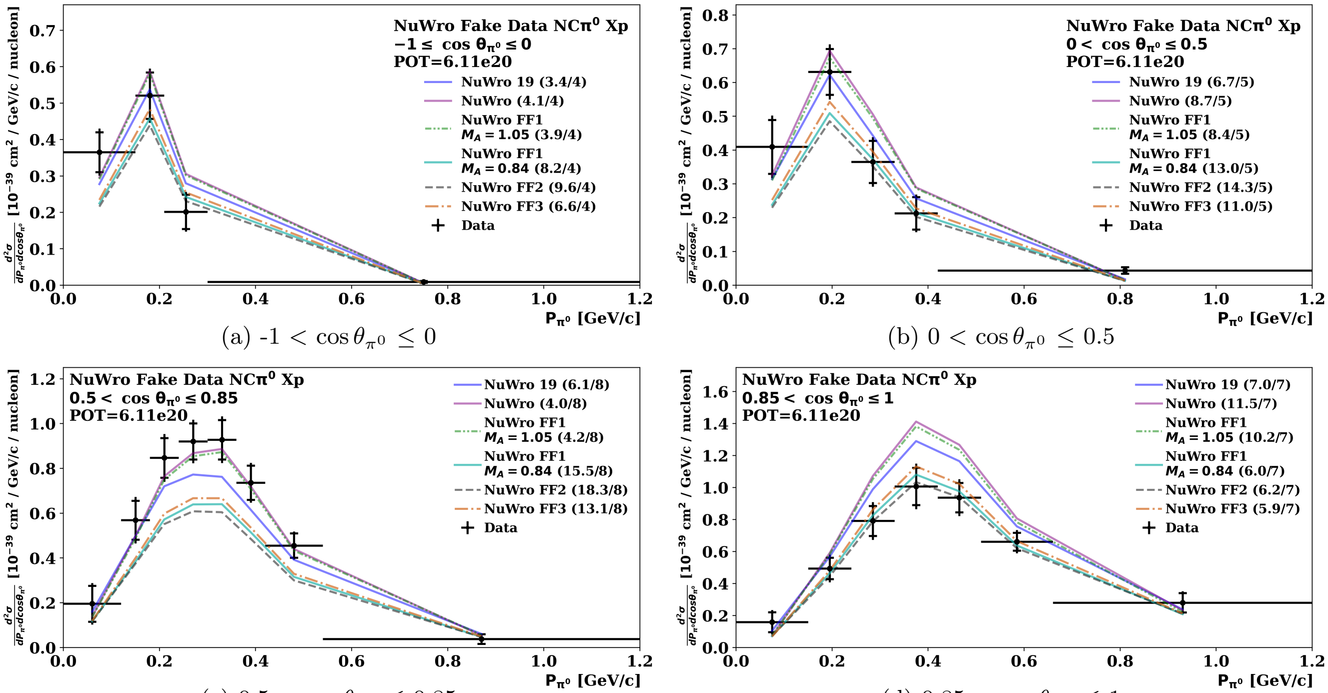


(a) -1 < $\cos\theta_{\pi^0}$ ≤ 0

(b) 0 < $\cos\theta_{\pi^0}$ ≤ 0.5

(c) 0.5 < $\cos\theta_{\pi^0}$ ≤ 0.85

(d) 0.85 < $\cos\theta_{\pi^0}$ ≤ 1

FIG. 43: Same as Fig. 39, but with the generator predictions from Fig. 2 of the main text that modify the form factors describing the neutrino-nucleon Δ excitation cross section.

## VII. ADDITIONAL MEASUREMENTS AND $\chi^2$ VALUES

Figure 44 shows the 0p and Np $\cos\theta_{\pi^0}$ differential cross section results analogous to the 0p and Np $P_{\pi^0}$ result shown in Fig. 1 of the main text. Sensitivity to the modeling of coherent pion production is illustrated by comparing these results to NEUT and GENIEv3 predictions with and without the coherent (COH) contribution. A prediction from GiBUU, which does not simulate coherent events, is also shown with and without the addition of the coherent prediction from NEUT. Because coherent events occur with small momentum transfer and leave the nucleus intact [10, 11], the impact of coherent pion production on the NC$\pi^0$ channel is only apparent for the 0p channel in the forward direction and the predictions with coherent events are slightly favored by the data. This is most noticeable for GiBUU, which underpredicts the most forward bins by almost 2$\sigma$ until the coherent prediction from NEUT is added. The resulting prediction falls within 1$\sigma$ of the data on all bins and the $\chi^2/ndf$ is lowered by about 0.5 thereby demonstrating the importance of properly modeling coherent interactions in describing NC$\pi^0$ production without protons in the final state. Characterizing the coherent process in more detail is beyond the scope of this work and could be explored by a future measurement with an event selection and analysis strategy tailored to disentangle resonant and coherent $\pi^0$ production.

Analogous to the simultaneous 0p and Np measurements seen in Fig. 1 of the main text and Fig. 44 of the supplemental material, the single-differential $P_{\pi^0}$ and $\cos\theta_{\pi^0}$ Xp cross section measurements are presented in this section. The $P_{\pi^0}$ result can be seen in Fig. 45a and the $\cos\theta_{\pi^0}$ result can be seen in Fig. 45b. These results are compared to predictions from the various generators described in the main text without any modification to their default parameters.

The single-differential Xp results show a similar set of trends as the results in the main text. For $P_{\pi^0}$, the sharper drop beyond the peak of the distribution around the 200-500 MeV range is caused by the energy dependence of pion reabsorption through the Δ resonance during FSI [12] is quite obvious. In this regime, GiBUU is the only generator not overpredicting the data and describes the data quite well, possibly due to its more robust description of FSI. However, GiBUU underestimated the cross section around the peak of the distribution, where the other generators describe the data well. This gives NEUT the lowest $\chi^2$ values, which other than slightly overpredicting in the 200-500 MeV range, shows very good agreement with the data. The GENIEv2 prediction is significantly worse than the other generators

due to its larger overprediction in the aforementioned regions which are more sensitive to FSI.

For the unfolded Xp $\cos\theta_{\pi^0}$ differential cross section result, `NEUT` agrees well at backwards angles and describes the rise in the cross section at forward angles quite well leading to a lower $\chi^2$ than achieved by the other generators. The two `GENIE`-based generator predictions overestimate this rise, and `GiBUU` underpredicts it. The former effect is possibly due to insufficient $\pi^0$ FSI, and the latter is possible in part due to the lack of coherent pion production in `GiBUU`. The discrepancy at forward angles is worst for `GENIEv2`, as is evident by its higher $\chi^2$, with the other three generators, which have comparable $\chi^2$ values, albeit larger than the one for `NEUT`.

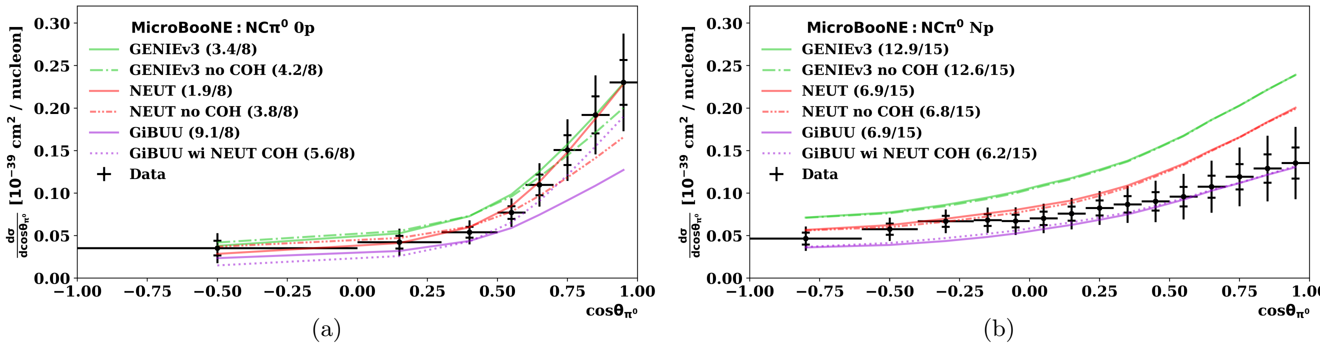


(a) (b)

FIG. 44: Unfolded 0p (a) and Np (b) $\cos\theta_{\pi^0}$ differential cross sections. The black inner (outer) error bars on the data points represent the statistical (total) uncertainties on the extracted cross section corresponding to the square root of the diagonal elements of the extracted covariance matrix. Generator predictions are indicated by the colored lines with corresponding $\chi^2/ndf$ values displayed in the legend.

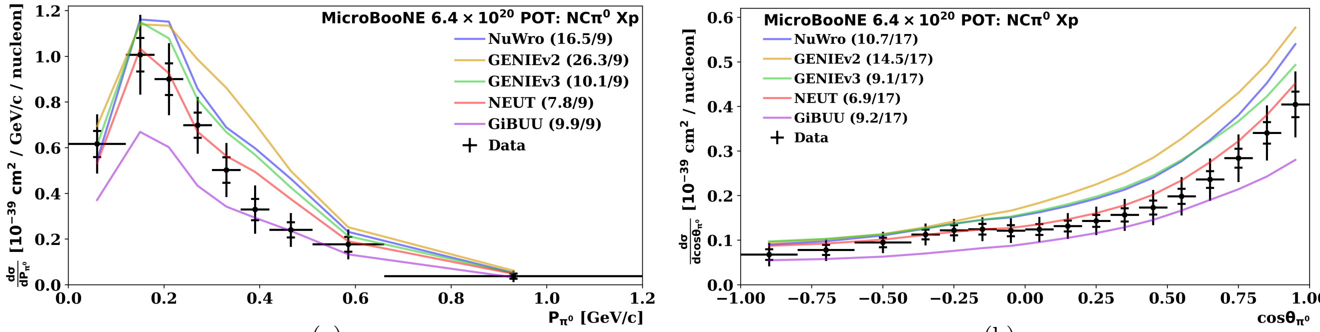


(a) (b)

FIG. 45: Unfolded Xp $P_{\pi^0}$ differential cross section result (a) and $\cos\theta_{\pi^0}$ differential cross section result (b). The black inner (outer) error bars on the data points represent the statistical (total) uncertainties on the extracted cross section corresponding to the square root of the diagonal elements of the extracted covariance matrix. Different generator predictions are indicated by the colored lines with corresponding $\chi^2$ values displayed in the legend.

Tables I and II contain additional $\chi^2$ values quantifying the various generator predictions' ability to describe the data. Generator predictions with the default parameters are shown in Table I and predictions with modified parameterizations of the $\Delta$ excitation form factors are shown in Table II. These tables include $\chi^2$ values calculated across the simultaneously measured 0p and Np bins, as well as for individual slices in the double-differential measurement. Additionally, the inter-variable correlations obtained with the blockwise unfolding [13] are used to calculate $\chi^2$ values across different measurements. These are listed in the "All Bins" columns. The covariance matrix used to produce these $\chi^2$ values is reported in the data release in `cov.txt`. More details on the data release are found in Sec. IX.

| Measurement | Channel | *ndf* | `NuWro` | `GENIEv2` | `GENIEv3` | `NEUT` | `GiBUU` |
|---|---|---|---|---|---|---|---|
| $P_{\pi^0}$ | 0p | 6 | 7.8 | 9.0 | 6.7 | 7.3 | 12.9 |
| | Np | 6 | 11.3 | 23.2 | 14.8 | 9.3 | 8.2 |
| | 0pNp | 12 | 16.0 | 28.0 | 18.8 | 13.2 | 17.0 |
| | Xp | 9 | 16.5 | 26.3 | 10.1 | 7.8 | 9.9 |
| $\cos\theta_{\pi^0}$ | 0p | 8 | 5.0 | 6.8 | 3.4 | 1.9 | 9.1 |
| | Np | 15 | 9.1 | 15.8 | 12.9 | 6.9 | 6.9 |
| | 0pNp | 23 | 11.3 | 18.3 | 18.7 | 10.5 | 14.6 |
| | Xp | 17 | 10.7 | 14.5 | 9.1 | 6.9 | 9.2 |
| $\{\cos\theta_{\pi^0}, P_{\pi^0}\}$ | Xp | 24 | 25.3 | 34.2 | 16.5 | 13.3 | 18.0 |
| $-1 > \cos\theta_{\pi^0} < 0$ | | 4 | 4.7 | 8.0 | 2.1 | 0.4 | 5.6 |
| $0 > \cos\theta_{\pi^0} < 0.5$ | | 5 | 4.3 | 7.7 | 3.0 | 0.4 | 4.3 |
| $0.5 > \cos\theta_{\pi^0} < 0.85$ | | 8 | 11.0 | 13.7 | 7.8 | 4.5 | 6.5 |
| $0.85 > \cos\theta_{\pi^0} < 1$ | | 7 | 14.9 | 9.7 | 6.2 | 6.5 | 6.8 |
| All Bins | 0p | 14 | 12.2 | 17.4 | 14.6 | 10.7 | 16.8 |
| | Np | 21 | 16.9 | 30.3 | 20.0 | 14.0 | 13.8 |
| | 0pNp | 35 | 24.5 | 39.9 | 30.3 | 23.0 | 28.9 |
| | Xp | 50 | 36.0 | 44.1 | 25.0 | 23.6 | 27.7 |
| | 0pNpXp | 85 | 82.2 | 68.8 | 47.8 | 53.9 | 58.5 |

TABLE I: Summary of the comparisons between the various generator prediction and each data result. When applicable, the 0p, Np, 0pNp and Xp $\chi^2$ and respective *ndf* are shown for each measured variable. Additional $\chi^2$ values including multiple measurements calculated using the covariance matrix obtained from the blockwise unfolding are also shown.

| Measurement | Channel | *ndf* | `NuWro` | `NuWro FF1` $M_A = 1.05$ | `NuWro FF1` $M_A = 0.84$ | `NuWro FF2` | `NuWro FF3` |
|---|---|---|---|---|---|---|---|
| $P_{\pi^0}$ | 0p | 6 | 7.8 | 7.5 | 6.4 | 6.7 | 6.2 |
| | Np | 6 | 11.3 | 10.8 | 6.8 | 6.4 | 6.9 |
| | 0pNp | 12 | 16.0 | 15.6 | 12.1 | 12.2 | 12.0 |
| | Xp | 9 | 16.5 | 15.9 | 10.7 | 10.6 | 11.0 |
| $\cos\theta_{\pi^0}$ | 0p | 8 | 5.0 | 4.5 | 3.0 | 3.3 | 2.8 |
| | Np | 15 | 9.1 | 8.5 | 5.6 | 5.8 | 5.9 |
| | 0pNp | 23 | 11.3 | 10.7 | 7.9 | 8.1 | 8.0 |
| | Xp | 17 | 10.7 | 10.2 | 6.9 | 7.0 | 7.1 |
| $\{\cos\theta_{\pi^0}, P_{\pi^0}\}$ | Xp | 24 | 25.3 | 24.1 | 17.0 | 16.9 | 17.7 |
| $-1 > \cos\theta_{\pi^0} < 0$ | | 4 | 4.7 | 4.1 | 1.2 | 1.4 | 1.2 |
| $0 > \cos\theta_{\pi^0} < 0.5$ | | 5 | 4.3 | 3.6 | 0.8 | 0.9 | 0.8 |
| $0.5 > \cos\theta_{\pi^0} < 0.85$ | | 8 | 11.0 | 10.2 | 5.5 | 5.5 | 5.8 |
| $0.85 > \cos\theta_{\pi^0} < 1$ | | 7 | 14.9 | 13.6 | 7.1 | 6.6 | 8.0 |
| All Bins | 0p | 14 | 12.2 | 11.6 | 8.8 | 9.1 | 8.8 |
| | Np | 21 | 16.9 | 16.3 | 11.7 | 11.5 | 12.1 |
| | 0pNp | 35 | 24.5 | 23.9 | 20.6 | 21.0 | 20.7 |
| | Xp | 50 | 36.0 | 35.2 | 28.6 | 28.7 | 29.0 |
| | 0pNpXp | 85 | 82.2 | 84.3 | 66.7 | 63.5 | 70.9 |

TABLE II: Summary of the comparisons between the generator predictions with different form factors and each data result. When applicable, the 0p, Np, 0pNp and Xp $\chi^2$ and respective *ndf* are shown for each measured variable. Additional $\chi^2$ values including multiple measurements calculated using the covariance matrix obtained from the blockwise unfolding are also shown.

## VIII. FORM FACTORS

What follows is a description of the predictions that utilize modified form factors. The evolution of $C_A$ as a function of $Q^2$ is shown for each prediction in Fig. 46. The `NuWro` prediction corresponds to a dipole form factor:

$$C_5^A(Q^2) = C_5^A(0)\frac{1}{\left(1+Q^2/M_A^2\right)^2} \tag{11}$$

with $M_A = 0.94$ GeV and $C_5^A(0) = 1.19$ as obtained by fits to ANL and BNL bubble chamber data in [14]. This is equivalent to the default used in the `NuWro` event generator. A second set of parameterizations, which utilize a modified dipole form factor,

$$C_5^A(Q^2) = C_5^A(0)\frac{1}{\left(1+Q^2/M_A^2\right)^2}\frac{1}{\left(1+Q^2/3M_A^2\right)} \tag{12}$$

are taken from [15]. Two values of with $M_A$ are considered; $M_A = 1.05$ GeV and $M_A = 0.84$ GeV. These predictions use $C_5^A(0) = 1.2$ and correspond to `NuWro FF1` $\mathtt{M_A}$`=1.05` and `NuWro FF1` $\mathtt{M_A}$`=0.84`, respectively. Additionally, as in [15], two other form factors with a steeper $Q^2$ dependence are also explored. These are

$$C_5^A(Q^2) = C_5^A(0)\frac{1}{\left(1+Q^2/M_A^2\right)^2}\frac{1}{\left(1+2Q^2/M_A^2\right)} \tag{13}$$

with $M_A = 1.05$ GeV, and

$$C_5^A(Q^2) = C_5^A(0)\frac{1}{\left(1+Q^2/M_A^2\right)^2}\frac{1}{\left(1+Q^2/3M_A^2\right)^2} \tag{14}$$

with $M_A = 0.95$ GeV. These parameterizations correspond to the `NuWro FF2` and `NuWro FF3`, respectively. These predictions also use $C_5^A(0) = 1.2$.

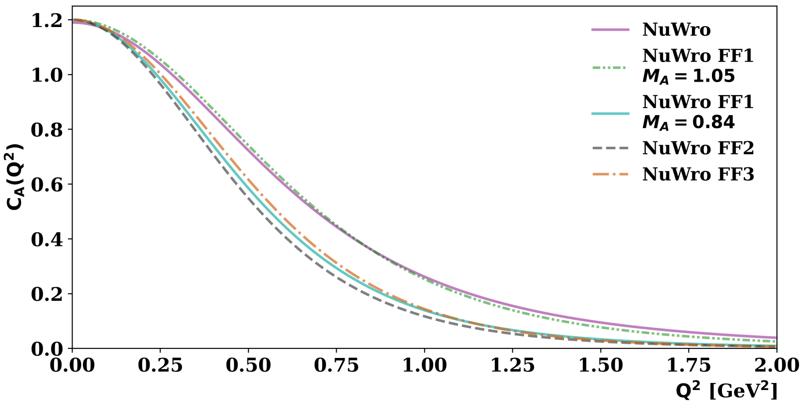


FIG. 46: The evolution of $C_A$ as a function of $Q^2$ for the various `NuWro` predictions with different parameterizations of the $\Delta$ excitation form factors.

## IX. DATA RELEASE

The unfolded cross section results shown in the main text and Sec. VII can be found tabulated below. The total uncertainty, corresponding to the square root of the diagonal elements of the extracted covariance matrix, is shown for each bin. The extracted cross section results and corresponding covariance matrices can be found in a machine-readable form in `xs.txt` and `cov.txt`, respectively. The additional smearing matrix, $A_C$, obtained from the Wiener-SVD unfolding can be found in the same format in `Ac.txt`. Any theory or event generator prediction should be multiplied by the additional smearing matrix when comparing to this data. These files are presented in a blockwise fashion with inter-variable correlations obtained via the blockwise unfolding procedure described in Sec. III B of [2]. The Global Bin index listed in the following tables corresponds to the location of the bin in the blockwise covariance matrix and the Bin index corresponds to the location within the given measurement. An example script demonstrating how to compare the data to an external prediction is also included. This script loads the various data release files into `ROOT TMatrixD` and `TVectorD` objects. It then compares the data to an external prediction contained in `pred.txt`, which in this case is the $\mu$`BooNE` tune MC, by first smearing the prediction and then calculating $\chi^2$ values for various measurements. More information on the files and their usage can be found in `readme.txt`.

The nominal $\nu_\mu$, $\bar{\nu}_\mu$, $\nu_e$, $\bar{\nu}_e$ fluxes of the Fermilab Booster Neutrino Beam (BNB) at the MicroBooNE detector location can be found in `numu_flux.txt`, `numubar_flux.txt`, `nue_flux.txt`, and `nuebar_flux.txt`, respectively. The integrated flux is calculated separately for all four neutrino flavors. The sum of these integrated fluxes is the flux constant that these results are averaged over. The total integrated flux and the fraction of the total integrated flux for each neutrino flavor is summarized in Table. III. Neutrino flux uncertainties are fully accounted for in the extracted covariance matrix and do not need to be included in theory or event generator predictions when comparing to the results. More information on the flux files can be found in `readme.txt`.

| Flavor | Total Flux | Fraction |
|---|---|---|
| $\nu_\mu$ | $4.585\times10^{11}$ | 0.9365 |
| $\bar{\nu}_\mu$ | $2.834\times10^{10}$ | 0.0579 |
| $\nu_e$ | $2.473\times10^{9}$ | 0.0051 |
| $\bar{\nu}_e$ | $2.508\times10^{8}$ | 0.0005 |
| **Total** | $4.896\times10^{11}$ | 1 |

TABLE III: The integrated nominal flux of the BNB for each neutrino flavor in units of number of neutrinos per $cm^2$ for an exposure of $6.369\times10^{20}$ protons on target. This is the reference flux the extracted cross section results are averaged over. The Fraction column corresponds to the fraction of the total flux produced by the given flavor.

| 0pNp $P_{\pi^0}$ differential cross section results | | | | | |
|---|---|---|---|---|---|
| Global Bin | Bin | $P_{\pi^0}$ Low (GeV/c) | $P_{\pi^0}$ High (GeV/c) | $\frac{d\sigma}{dP_{\pi^0}}$ $\left(\times 10^{-39} \frac{\text{cm}^2}{\text{nucleon (GeV/c)}}\right)$ | Uncertainty $\left(\times 10^{-39} \frac{\text{cm}^2}{\text{nucleon (GeV/c)}}\right)$ |
| 0p | | | | | |
| 0 | 0 | 0.0 | 0.15 | 0.4469 | 0.0796 |
| 1 | 1 | 0.15 | 0.21 | 0.5744 | 0.0940 |
| 2 | 2 | 0.21 | 0.3 | 0.4328 | 0.0765 |
| 3 | 3 | 0.3 | 0.42 | 0.2809 | 0.0505 |
| 4 | 4 | 0.42 | 0.6 | 0.1241 | 0.0353 |
| 5 | 5 | 0.6 | 1.2 | 0.0232 | 0.0156 |
| Np | | | | | |
| 6 | 6 | 0.0 | 0.12 | 0.2101 | 0.0856 |
| 7 | 7 | 0.12 | 0.18 | 0.5026 | 0.1269 |
| 8 | 8 | 0.18 | 0.3 | 0.3660 | 0.0853 |
| 9 | 9 | 0.3 | 0.42 | 0.1996 | 0.0644 |
| 10 | 10 | 0.42 | 0.6 | 0.0426 | 0.0396 |
| 11 | 11 | 0.6 | 1.2 | 0.0241 | 0.0164 |

TABLE IV: Unfolded 0pNp $P_{\pi^0}$ differential cross section results. The uncertainty corresponds to the square root of the diagonal elements of the extracted covariance matrix. Bin corresponds to the bin index within the given measurement, and Global Bin corresponds to the bin index within the blockwise covariance matrix.

| Xp $P_{\pi^0}$ differential cross section result | | | | | |
|---|---|---|---|---|---|
| Global Bin | Bin | $P_{\pi^0}$ Low (GeV/c) | $P_{\pi^0}$ High (GeV/c) | $\frac{d\sigma}{dP_{\pi^0}}$ $\left(\times 10^{-39} \frac{\text{cm}^2}{\text{nucleon GeV/c}}\right)$ | Uncertainty $\left(\times 10^{-39} \frac{\text{cm}^2}{\text{nucleon GeV/c}}\right)$ |
| 12 | 0 | 0.0 | 0.12 | 0.6168 | 0.1300 |
| 13 | 1 | 0.12 | 0.18 | 1.0073 | 0.1751 |
| 14 | 2 | 0.18 | 0.24 | 0.9004 | 0.1578 |
| 15 | 3 | 0.24 | 0.3 | 0.6987 | 0.1244 |
| 16 | 4 | 0.3 | 0.36 | 0.5026 | 0.1187 |
| 17 | 5 | 0.36 | 0.42 | 0.3295 | 0.1055 |
| 18 | 6 | 0.42 | 0.51 | 0.2406 | 0.0742 |
| 19 | 7 | 0.51 | 0.66 | 0.1771 | 0.0655 |
| 20 | 8 | 0.66 | 1.2 | 0.0378 | 0.0261 |

TABLE V: Unfolded Xp $P_{\pi^0}$ differential cross section result. The uncertainty corresponds to the square root of the diagonal elements of the extracted covariance matrix. Bin corresponds to the bin index within the given measurement, and Global Bin corresponds to the bin index within the blockwise covariance matrix.

| 0pNp $\cos\theta_{\pi^0}$ differential cross section results | | | | | |
|---|---|---|---|---|---|
| Global Bin | Bin | $\cos\theta_{\pi^0}$ Low | $\cos\theta_{\pi^0}$ High | $\frac{d\sigma}{d\cos\theta_{\pi^0}}$ $\left(\times 10^{-39} \frac{\text{cm}^2}{\text{nucleon}}\right)$ | Uncertainty $\left(\times 10^{-39} \frac{\text{cm}^2}{\text{nucleon}}\right)$ |
| 0p | | | | | |
| 21 | 0 | -1 | 0 | 0.0354 | 0.0177 |
| 22 | 1 | 0 | 0.3 | 0.0423 | 0.0159 |
| 23 | 2 | 0.3 | 0.5 | 0.0539 | 0.0141 |
| 24 | 3 | 0.5 | 0.6 | 0.0771 | 0.0167 |
| 25 | 4 | 0.6 | 0.7 | 0.1097 | 0.0255 |
| 26 | 5 | 0.7 | 0.8 | 0.1507 | 0.0362 |
| 27 | 6 | 0.8 | 0.9 | 0.1921 | 0.0465 |
| 28 | 7 | 0.9 | 1 | 0.2303 | 0.0574 |
| Np | | | | | |
| 29 | 8 | -1 | -0.6 | 0.0465 | 0.0144 |
| 30 | 9 | -0.6 | -0.4 | 0.0575 | 0.0138 |
| 31 | 10 | -0.4 | -0.2 | 0.0669 | 0.0139 |
| 32 | 11 | -0.2 | -0.1 | 0.0683 | 0.0149 |
| 33 | 12 | -0.1 | 0 | 0.0671 | 0.0162 |
| 34 | 13 | 0 | 0.1 | 0.0703 | 0.0174 |
| 35 | 14 | 0.1 | 0.2 | 0.0758 | 0.0185 |
| 36 | 15 | 0.2 | 0.3 | 0.0826 | 0.0199 |
| 37 | 16 | 0.3 | 0.4 | 0.0868 | 0.0217 |
| 38 | 17 | 0.4 | 0.5 | 0.0903 | 0.0243 |
| 39 | 18 | 0.5 | 0.6 | 0.0959 | 0.0269 |
| 40 | 19 | 0.6 | 0.7 | 0.1076 | 0.0307 |
| 41 | 20 | 0.7 | 0.8 | 0.1193 | 0.0346 |
| 42 | 21 | 0.8 | 0.9 | 0.1290 | 0.0386 |
| 43 | 22 | 0.9 | 1 | 0.1355 | 0.0425 |

TABLE VI: Unfolded 0pNp $\cos\theta_{\pi^0}$ differential cross section results. The uncertainty corresponds to the square root of the diagonal elements of the extracted covariance matrix. Bin corresponds to the bin index within the given measurement, and global bin corresponds to the bin index within the blockwise covariance matrix.

| Xp $\cos\theta_{\pi^0}$ differential cross section results | | | | | |
|---|---|---|---|---|---|
| Global Bin | Bin | $\cos\theta_{\pi^0}$ Low | $\cos\theta_{\pi^0}$ High | $\frac{d\sigma}{d\cos\theta_{\pi^0}}$ $\left(\times 10^{-39}\,\frac{\text{cm}^2}{\text{nucleon}}\right)$ | Uncertainty $\left(\times 10^{-39}\,\frac{\text{cm}^2}{\text{nucleon}}\right)$ |
| 44 | 0 | -1 | -0.8 | 0.0680 | 0.0265 |
| 45 | 1 | -0.8 | -0.6 | 0.0784 | 0.0249 |
| 46 | 2 | -0.6 | -0.4 | 0.0952 | 0.0239 |
| 47 | 3 | -0.4 | -0.3 | 0.1129 | 0.0246 |
| 48 | 4 | -0.3 | -0.2 | 0.1224 | 0.0255 |
| 49 | 5 | -0.2 | -0.1 | 0.1248 | 0.0269 |
| 50 | 6 | -0.1 | 0 | 0.1214 | 0.0276 |
| 51 | 7 | 0 | 0.1 | 0.1242 | 0.0282 |
| 52 | 8 | 0.1 | 0.2 | 0.1319 | 0.0291 |
| 53 | 9 | 0.2 | 0.3 | 0.1435 | 0.0320 |
| 54 | 10 | 0.3 | 0.4 | 0.1570 | 0.0360 |
| 55 | 11 | 0.4 | 0.5 | 0.1734 | 0.0395 |
| 56 | 12 | 0.5 | 0.6 | 0.1986 | 0.0431 |
| 57 | 13 | 0.6 | 0.7 | 0.2364 | 0.0477 |
| 58 | 14 | 0.7 | 0.8 | 0.2841 | 0.0533 |
| 59 | 15 | 0.8 | 0.9 | 0.3409 | 0.0618 |
| 60 | 16 | 0.9 | 1 | 0.4047 | 0.0739 |

TABLE VII: Unfolded Xp $\cos\theta_{\pi^0}$ differential cross section results. The uncertainty corresponds to the square root of the diagonal elements of the extracted covariance matrix. Bin corresponds to the bin index within the given measurement, and Global Bin corresponds to the bin index within the blockwise covariance matrix.

| Xp $\cos\theta_{\pi^0}$ and $P_{\pi^0}$ double-differential cross section result | | | | | | | |
|---|---|---|---|---|---|---|---|
| Global Bin | Bin | $\cos\theta_{\pi^0}$ Low | $\cos\theta_{\pi^0}$ High | $P_{\pi^0}$ Low (GeV/c) | $P_{\pi^0}$ High (GeV/c) | $\frac{d^2\sigma}{dP_{\pi^0}\,d\cos\theta_{\pi^0}}$ $\left(\times10^{-39}\frac{\text{cm}^2}{\text{nucleon (GeV/c)}}\right)$ | Uncertainty $\left(\times10^{-39}\frac{\text{cm}^2}{\text{nucleon (GeV/c)}}\right)$ |
| 61 | 0 | -1 | 0 | 0 | 0.15 | 0.3010 | 0.0917 |
| 62 | 1 | -1 | 0 | 0.15 | 0.21 | 0.4274 | 0.0890 |
| 63 | 2 | -1 | 0 | 0.21 | 0.3 | 0.2204 | 0.0702 |
| 64 | 3 | -1 | 0 | 0.3 | 1.2 | 0.0085 | 0.0042 |
| 65 | 4 | 0 | 0.5 | 0 | 0.15 | 0.2407 | 0.1023 |
| 66 | 5 | 0 | 0.5 | 0.15 | 0.24 | 0.3964 | 0.1014 |
| 67 | 6 | 0 | 0.5 | 0.24 | 0.33 | 0.2985 | 0.0797 |
| 68 | 7 | 0 | 0.5 | 0.33 | 0.42 | 0.1983 | 0.0551 |
| 69 | 8 | 0 | 0.5 | 0.42 | 1.2 | 0.0176 | 0.0068 |
| 70 | 9 | 0.5 | 0.85 | 0 | 0.12 | 0.4589 | 0.1407 |
| 71 | 10 | 0.5 | 0.85 | 0.12 | 0.18 | 0.6683 | 0.1757 |
| 72 | 11 | 0.5 | 0.85 | 0.18 | 0.24 | 0.7095 | 0.1663 |
| 73 | 12 | 0.5 | 0.85 | 0.24 | 0.3 | 0.6670 | 0.1501 |
| 74 | 13 | 0.5 | 0.85 | 0.3 | 0.36 | 0.5485 | 0.1555 |
| 75 | 14 | 0.5 | 0.85 | 0.36 | 0.42 | 0.3718 | 0.1397 |
| 76 | 15 | 0.5 | 0.85 | 0.42 | 0.54 | 0.1987 | 0.0881 |
| 77 | 16 | 0.5 | 0.85 | 0.54 | 1.2 | 0.0875 | 0.0298 |
| 78 | 17 | 0.85 | 1 | 0 | 0.15 | 0.2704 | 0.1296 |
| 79 | 18 | 0.85 | 1 | 0.15 | 0.24 | 0.5218 | 0.1329 |
| 80 | 19 | 0.85 | 1 | 0.24 | 0.33 | 0.7079 | 0.1853 |
| 81 | 20 | 0.85 | 1 | 0.33 | 0.42 | 0.8002 | 0.2342 |
| 82 | 21 | 0.85 | 1 | 0.42 | 0.51 | 0.6722 | 0.1900 |
| 83 | 22 | 0.85 | 1 | 0.51 | 0.66 | 0.4258 | 0.1056 |
| 84 | 23 | 0.85 | 1 | 0.66 | 1.2 | 0.1464 | 0.0986 |

TABLE VIII: Unfolded Xp $\cos\theta_{\pi^0}$ and $P_{\pi^0}$ double-differential cross section result. The uncertainty corresponds to the square root of the diagonal elements of the extracted covariance matrix. Bin corresponds to the bin index within the given measurement, and Global Bin corresponds to the bin index within the blockwise covariance matrix.


[1] M. L. Eaton, *Multivariate Statistics: a Vector Space Approach* (John Wiley and Sons, 1983) pp. 116–117.

[2] P. Abratenko *et al.* (MicroBooNE Collaboration), Inclusive cross section measurements in final states with and without protons for charged-current $\nu_\mu$-Ar scattering in MicroBooNE, arXiv preprint (2024), arXiv:2402.19216 [hep-ex].

[3] P. Abratenko *et al.* (MicroBooNE Collaboration), First Measurement of Energy-Dependent Inclusive Muon Neutrino Charged-Current Cross Sections on Argon with the MicroBooNE Detector, Phys. Rev. Lett. **128**, 151801 (2022).

[4] P. Abratenko *et al.* (MicroBooNE Collaboration), Search for an anomalous excess of inclusive charged-current $\nu_e$ interactions in the MicroBooNE experiment using Wire-Cell reconstruction, Phys. Rev. D **105**, 112005 (2022).

[5] P. Abratenko *et al.* (MicroBooNE Collaboration), Measurement of triple-differential inclusive muon-neutrino charged-current cross section on argon with the MicroBooNE detector (2023), arXiv:2307.06413 [hep-ex].

[6] P. Abratenko *et al.* (MicroBooNE Collaboration), First simultaneous measurement of differential muon-neutrino charged-current cross sections on argon for final states with and without protons using MicroBooNE data, arXiv preprint (2024),

arXiv:2402.19281 [hep-ex].

[7] L. Alvarez-Ruso *et al.* (GENIE Collaboration), Recent highlights from GENIE v3, Eur. Phys. J. ST **230**, 4449 (2021).

[8] Y. Hayato and L. Pickering, The NEUT neutrino interaction simulation program library, Eur. Phys. J. ST **230**, 4469 (2021).

[9] P. Stowell *et al.*, NUISANCE: a neutrino cross-section generator tuning and comparison framework, J. Instrum. **12** (01), P01016.

[10] L. Alvarez-Ruso, Review of weak coherent pion production, AIP Conf. Proc. **1405**, 140 (2011).

[11] D. Rein and L. M. Sehgal, Coherent $\pi^0$ production in neutrino reactions, Nucl. Phys. B **223**, 29 (1983).

[12] T. Leitner, L. Alvarez-Ruso, and U. Mosel, Neutral current neutrino-nucleus interactions at intermediate energies, Phys. Rev. C **74**, 065502 (2006).

[13] S. Gardiner, Mathematical methods for neutrino cross-section extraction, arXiv preprint (2024), FERMILAB-PUB-23-692-CSAID, arXiv:2401.04065 [hep-ex].

[14] K. M. Graczyk, D. Kiełczewska, P. Przewłocki, and J. T. Sobczyk, $C_5^A$ axial form factor from bubble chamber experiments, Phys. Rev. D **80**, 093001 (2009).

[15] O. Lalakulich and E. A. Paschos, Resonance production by neutrinos: $J = 3/2$ resonances, Phys. Rev. D **71**, 074003 (2005).
